# Supplementary material for: Determination of Nano-sized Adsorbate Mass in Solution using Mechanical Resonators: Elimination of the so far Inseparable Liquid Contribution
Source: arXiv:2010.12414 ancillary file (2021-05-08)
Supplement: Supplementary file 1 [file Armanious_et_al_SI.pdf]

# Supporting Information for Determination of Adsorbate Mass in Solution using Mechanical Resonators: Elimination of the Inseparable Liquid Contribution

Antonius Armanious\*<sup>†1</sup>, Björn Agnarsson<sup>1</sup>, Anders Lundgren<sup>2</sup>, Vladimir P. Zhdanov<sup>1,3</sup>,  
and Fredrik Höök\*<sup>1</sup>

<sup>1</sup>Division of Nano and Biological Physics, Department of Physics, Chalmers University of  
Technology, Gothenburg, Sweden

<sup>2</sup>Department of Chemistry and Molecular Biology, University of Gothenburg, Gothenburg,  
Sweden

<sup>3</sup>Boriskov Institute of Catalysis, Russian Academy of Sciences, Novosibirsk, Russia

---

## Table of Contents

---

|     |                                                                                                 |    |
|-----|-------------------------------------------------------------------------------------------------|----|
| S1  | Materials and Methods                                                                           | 2  |
| S2  | Physical properties of D <sub>2</sub> O/H <sub>2</sub> O and glycerol/H <sub>2</sub> O mixtures | 4  |
| S3  | Measuring QCM response from different liquids on flat substrates                                | 6  |
| S4  | QCM response due to adsorption of NPs in different liquids and in air                           | 7  |
| S5  | Independent determination of the mass of adsorbed NPs                                           | 10 |
| S6  | Theoretical basis for the coupled-liquid response of QCM                                        | 14 |
| S7  | QCM response with reference to air                                                              | 16 |
| S8  | Low charge density of silanized SiO <sub>2</sub> sensors                                        | 21 |
| S9  | Effect of D <sub>2</sub> O concentration on the measured and extrapolated responses             | 22 |
| S10 | Effect of the overtone number on the measured and extrapolated responses                        | 23 |
| S11 | Surface plasmon resonance results for humic acids adlayer                                       | 26 |

---

\*armanioa@ethz.ch; fredrik.hook@chalmers.se

<sup>†</sup>Present address: Laboratory of Food and Soft Materials, Department of Health Sciences and Technology,  
ETH Zürich, Zürich, Switzerland

# S1 Materials and Methods

## Chemicals & Materials

Ethanol ( $\geq 99.5\%$ ) was purchased from Solveco (Roserberg, Sweden). Sodium dodecyl sulfate (SDS;  $\geq 99.0\%$ ), anhydrous methanol (99.8%), glycerol ( $\geq 99\%$ ),  $D_2O$  (99.9 *atom % D*),  $DCl$  ( $\geq 99$  *atom % D*),  $NaOD$  (40 %wt.),  $HCl$  (1 *M*),  $NaCl$  ( $\geq 99\%$ ),  $CaCl_2$  anhydrous ( $\geq 93\%$ ), bis(2-hydroxyethyl)amino-tris-(hydroxymethyl)-methane (Bis-Tris;  $\geq 98\%$ ), citric acid monohydrate ( $\geq 98\%$ ), trisodium citrate dihydrate, poly-L-lysine (PLL; MW = 70000 – 150000), humic acids (HA), (3-aminopropyl)dimethylethoxysilane, 97%, and 150 nm  $SiO_2$  nanoparticles (NPs) were purchased from Merck Sigma-Aldrich (Darmstadt, Germany).

## Buffers

Three different buffers were used

- pH (pD) = 7.0, 150 mM  $NaCl$ , and 10 mM Bis-Tris
- pH (pD) = 7.0, 150 mM  $NaCl$ , 2.5 mM  $CaCl_2$ , and 10 mM Bis-Tris
- pH (pD) = 4.0,  $\approx 3.8$  mM trisodium citrate dihydrate and  $\approx 6.2$  mM citric acid monohydrate

Buffers were prepared in

- $H_2O$  (Milli-Q purity with resistivity  $\approx 18.2\ \Omega \cdot cm$ ; Merck Millipore, Molsheim, France)
- 100%, 80%, 60%, and 40% of  $D_2O$  in  $H_2O$  corresponding to a molar fraction of  $D_2O$ ,  $x_{D_2O} = 1.0, 0.8, 0.6, \& 0.4$ , respectively.
- 4.55%wt., 3.80%wt., 2.99%wt. and 2.12%wt. of glycerol in  $H_2O$  which match the kinematic viscosity,  $\nu$ , of 100%, 80%, 60%, and 40%  $D_2O$  solutions, respectively.
- 10.86%wt. of glycerol in  $H_2O$  which match the product of the density and viscosity,  $\rho\eta$ , of 100%  $D_2O$ .

The physical properties of all these solutions can be found in Table S1 in the SI.

The pH of buffers in  $H_2O$  and glycerol/ $H_2O$  mixtures were determined using a Mettler-Toledo (Ohaio, US) pH meter. The pH (pD) for  $D_2O$ -containing buffers were determined using pH paper, the color of which was compared and matched against the color of a similar pH paper after submerging in the corresponding  $H_2O$ -based buffer. This procedure was followed to make sure that the buffers prepared in  $H_2O$ ,  $D_2O$ ,  $D_2O/H_2O$  mixtures, or glycerol/ $H_2O$  mixtures had the same pH (pD). Note that buffer dissociation constants depend on the environment they are in; so the buffer will behave differently in  $H_2O$  than in a glycerol/ $H_2O$  mixture. For this reason, adding equal amounts of the chemicals does not guarantee having the same pH; it is therefore necessary to check and adjust the pH of each solution.

$H_2O$ -based buffers were either sterilized by autoclaving at 120 °C for 20 minutes or by sterile filtration using 0.22  $\mu m$  Stericup-GV Sterile Vacuum filters (Millipore, France); all other buffers were sterile filtered using 0.22  $\mu m$  Stericup-GV Sterile Vacuum filters (Millipore, France). Note that the buffers filtered through the 0.22  $\mu m$  Stericup-GV Sterile Vacuum filters caused aggregation of the  $SiO_2$  NPs, suggesting that the filter membrane released leachate in the buffer. This problem was addressed by either pre-washing the filters with buffer or autoclaving the buffers instead of filtering them, the later was only done for  $H_2O$ -based buffers.

## QCM experiments

The QCM experiments were conducted in an E4 system (Biolin, Sweden) coupled to GX-274 Autosampler (Gillson, USA) on AT-cut 5 MHz quartz sensors, coated with  $SiO_2$ . The sensors were either used without modification or after silanization with amine-terminated silanes. Bare sensors were cleaned by bath sonication for 15 minutes in 2%wt. SDS solution, followed by rinsing with Milli-Q water, then drying under a  $N_2$  flow, and finally treating with  $O_2$  plasma for 3 minutes directly before use. The temperature and flow rate was kept constant all through the QCM experiments at 25 °C and 50  $\mu l \cdot min^{-1}$ , respectively. At the end of the  $SiO_2$  NPs adsorption experiments, the solution in contact of the sensor was exchanged to ethanol  $\geq 99.5\%$ , then the sensors were dried *in-situ* under  $N_2$  flow and at temperature of 60 °C; finally the temperature were lowered down again to 25 °C. This procedure was followed to dry the sensors for determining the response after drying (in air) and for further analysis using AFM and SEM while minimizing any drying effects, such as aggregation of the NPs on the surface. A step-by-step experimental and calculation procedure are presented in Sections S3 and S4.

## Silanization of SiO<sub>2</sub> sensors

The sensors were first cleaned by: bath sonication for 15 minutes in 2 %wt. SDS solution, rinsing with MilliQ water, treating with O<sub>2</sub> plasma for 3 minutes, adding few drops of 4 M H<sub>2</sub>SO<sub>4</sub> on the surface of the sensor for 30 minutes, rinsing thoroughly under flowing MilliQ water, rinsing thoroughly using anhydrous methanol, and finally drying under N<sub>2</sub> flow. The sensors were then incubated in 7.5 %v/v 3-(Ethoxydimethylsilyl)propylamine in anhydrous methanol for at least 30 minutes. Afterwards the sensors were rinsed thoroughly with anhydrous methanol to avoid precipitation of the silanes which happens in the presence of water or ethanol. Finally the sensors are rinsed with MilliQ water and mounted in the instrument for use.

## Atomic Force Microscopy (AFM)

A Bruker Dimension 3100 scanning probe microscopy system was used for *ex-situ* atomic force imaging of the surface of dried QCM sensors. The height (z-distance) of the NPs were used to determine their size. A detailed experimental and computation procedure are presented in Section S5.

## Scanning Electron Microscopy (SEM)

Scanning electron microscopy (Zeiss Ultra 55 FEG, in-lens mode, ETH=2 kV) was used for general *ex-situ* characterization of the dried QCM sensor surfaces and for determination of NP surface coverage. Images were acquired at a location as close as possible to the center of the sensor; the area of the sensor which contributes the most to the QCM signal. We also tried to select an imaging area that did not show any visible drying effects, such as clear aggregation of the NPs. Based on the acquired images NPs were counted using ImageJ; the total number of the NPs was then divided by the area of the image to obtain the number of NPs per  $\mu\text{m}^2$ . Features much larger or much smaller than the size of the NPs were not counted towards the total number of the NPs. Features which showed a double layer of NPs was double counted. Examples of these different cases, as well as a detailed experimental and computation procedure are presented in Section S5 in the SI.

## Surface resonance plasmon (SPR) experiments

The SPR experiments were conducted using a dual wavelength, 670 and 785 nm, multi-parametric SPR Navi<sup>TM</sup>420A (BioNavis, Finland) on silica-coated sensors. The sensors were cleaned by bath sonication for 15 minutes in 2%wt. SDS solution, followed by rinsing with Milli-Q water, then drying under a N<sub>2</sub> flow, and finally treating in a UV/Ozone chamber for 45 minutes directly before use. The temperature and flow rate were kept constant at 25 °C and  $7 \mu\text{l} \cdot \text{min}^{-1}$ , respectively.

## S2 Physical properties of D<sub>2</sub>O/H<sub>2</sub>O and glycerol/H<sub>2</sub>O mixtures

Densities and viscosities of the D<sub>2</sub>O/H<sub>2</sub>O mixtures were determined using equations<sup>1</sup>

$$\rho_{\text{D}_2\text{O}/\text{H}_2\text{O}} = \frac{x_{\text{H}_2\text{O}} \cdot M_{\text{H}_2\text{O}} + x_{\text{D}_2\text{O}} \cdot M_{\text{D}_2\text{O}}}{x_{\text{H}_2\text{O}} \cdot M_{\text{H}_2\text{O}}/\rho_{\text{H}_2\text{O}} + x_{\text{D}_2\text{O}} \cdot M_{\text{D}_2\text{O}}/\rho_{\text{D}_2\text{O}}}, \quad (\text{S1})$$

$$\eta_{\text{D}_2\text{O}/\text{H}_2\text{O}} = x_{\text{H}_2\text{O}} \cdot \eta_{\text{H}_2\text{O}} + x_{\text{D}_2\text{O}} \cdot \eta_{\text{D}_2\text{O}}, \quad (\text{S2})$$

where:

- $\rho_{\text{D}_2\text{O}/\text{H}_2\text{O}}$  is the density of D<sub>2</sub>O/H<sub>2</sub>O mixture [ $\text{g} \cdot \text{cm}^{-3}$ ].
- $x_{\text{H}_2\text{O}}$  and  $x_{\text{D}_2\text{O}}$  are the molar fractions of H<sub>2</sub>O and D<sub>2</sub>O, respectively.
- $M_{\text{H}_2\text{O}}$  and  $M_{\text{D}_2\text{O}}$  are the molar masses of H<sub>2</sub>O and D<sub>2</sub>O, respectively;  $M_{\text{H}_2\text{O}} = 18.0152 \text{ g} \cdot \text{mol}^{-1}$  and  $M_{\text{D}_2\text{O}} = 20.0275 \text{ g} \cdot \text{mol}^{-1}$ .
- $\rho_{\text{H}_2\text{O}}$  and  $\rho_{\text{D}_2\text{O}}$  are the densities of H<sub>2</sub>O and D<sub>2</sub>O, respectively; at 25 °C,  $\rho_{\text{H}_2\text{O}} = 0.997 \text{ g} \cdot \text{cm}^{-3}$  and  $\rho_{\text{D}_2\text{O}} = 1.104 \text{ g} \cdot \text{cm}^{-3}$  (Ref. 2).
- $\eta_{\text{D}_2\text{O}/\text{H}_2\text{O}}$  is the viscosity of D<sub>2</sub>O/H<sub>2</sub>O mixture [ $\text{g} \cdot \text{cm}^{-1} \cdot \text{sec}^{-1}$ ].
- $\eta_{\text{H}_2\text{O}}$  and  $\eta_{\text{D}_2\text{O}}$  are the viscosities of H<sub>2</sub>O and D<sub>2</sub>O, respectively; at 25 °C,  $\eta_{\text{H}_2\text{O}} = 0.893 \text{ g} \cdot \text{cm}^{-1} \cdot \text{sec}^{-1}$  (Ref. 3) and  $\eta_{\text{D}_2\text{O}} = 1.094 \text{ g} \cdot \text{cm}^{-1} \cdot \text{sec}^{-1}$  (Ref. 1).

Densities and viscosities of the glycerol/H<sub>2</sub>O mixtures were obtained from Refs. 4 and 3. The physical properties of all the solutions are compiled in Table S1 and Fig. S1.

**Table S1: Physical properties of D<sub>2</sub>O/H<sub>2</sub>O<sup>1–5</sup> and glycerol/H<sub>2</sub>O<sup>4</sup> mixtures at 25 °C.** The data are grouped for each D<sub>2</sub>O/H<sub>2</sub>O mixture and their property matching glycerol/H<sub>2</sub>O mixtures, with all properties of D<sub>2</sub>O/H<sub>2</sub>O mixtures and the matched property of the corresponding glycerol/H<sub>2</sub>O mixtures shown in **bold**.

| Solution                                               | Kinematic Viscosity,<br>$\nu = \eta/\rho$ [ $10^{-2} \cdot \text{cm}^2 \cdot \text{sec}$ ] | Viscosity, $\eta$<br>[ $10^{-2} \cdot \text{g} \cdot \text{cm}^{-1} \cdot \text{sec}^{-1}$ ] | $\rho \cdot \eta$<br>[ $10^{-2} \cdot \text{g}^2 \cdot \text{cm}^{-4} \cdot \text{sec}^{-1}$ ] | Density, $\rho$<br>[ $\text{g} \cdot \text{cm}^{-3}$ ] |
|--------------------------------------------------------|--------------------------------------------------------------------------------------------|----------------------------------------------------------------------------------------------|------------------------------------------------------------------------------------------------|--------------------------------------------------------|
| 100% D <sub>2</sub> O/0% H <sub>2</sub> O <sup>a</sup> | <b>0.991</b>                                                                               | <b>1.094</b>                                                                                 | <b>1.208</b>                                                                                   | <b>1.104</b>                                           |
| 4.55%wt gly. in H <sub>2</sub> O <sup>b</sup>          | <b>0.991</b>                                                                               | 0.998                                                                                        | 1.006                                                                                          | 1.008                                                  |
| 10.86%wt gly. in H <sub>2</sub> O <sup>c</sup>         | 1.155                                                                                      | 1.181                                                                                        | <b>1.208</b>                                                                                   | 1.023                                                  |
| 80% D <sub>2</sub> O/20% H <sub>2</sub> O <sup>a</sup> | <b>0.973</b>                                                                               | <b>1.054</b>                                                                                 | <b>1.141</b>                                                                                   | <b>1.083</b>                                           |
| 3.80%wt gly. in H <sub>2</sub> O <sup>b</sup>          | <b>0.973</b>                                                                               | 0.979                                                                                        | 0.985                                                                                          | 1.006                                                  |
| 60% D <sub>2</sub> O/40% H <sub>2</sub> O <sup>a</sup> | <b>0.955</b>                                                                               | <b>1.014</b>                                                                                 | <b>1.076</b>                                                                                   | <b>1.062</b>                                           |
| 2.99%wt gly. in H <sub>2</sub> O <sup>b</sup>          | <b>0.955</b>                                                                               | 0.959                                                                                        | 0.963                                                                                          | 1.004                                                  |
| 40% D <sub>2</sub> O/60% H <sub>2</sub> O <sup>a</sup> | <b>0.936</b>                                                                               | <b>0.973</b>                                                                                 | <b>1.012</b>                                                                                   | <b>1.040</b>                                           |
| 2.12%wt gly. in H <sub>2</sub> O <sup>b</sup>          | <b>0.936</b>                                                                               | 0.938                                                                                        | 0.940                                                                                          | 1.002                                                  |
| 0% D <sub>2</sub> O/100% H <sub>2</sub> O              | <b>0.896</b>                                                                               | <b>0.893</b>                                                                                 | <b>0.890</b>                                                                                   | <b>0.997</b>                                           |

<sup>a</sup> 100%, 80%, 60%, 40%, 20%, and 0% correspond to the molar fractions 1.0, 0.8, 0.6, 0.4, 0.2, and 0 of D<sub>2</sub>O and/or H<sub>2</sub>O. <sup>b</sup> Kinematic viscosity matched glycerol/H<sub>2</sub>O mixture,  $\nu_{\text{matched}}$ .

<sup>c</sup> Density times viscosity matched glycerol/H<sub>2</sub>O mixture,  $(\rho\eta)_{\text{matched}}$ .

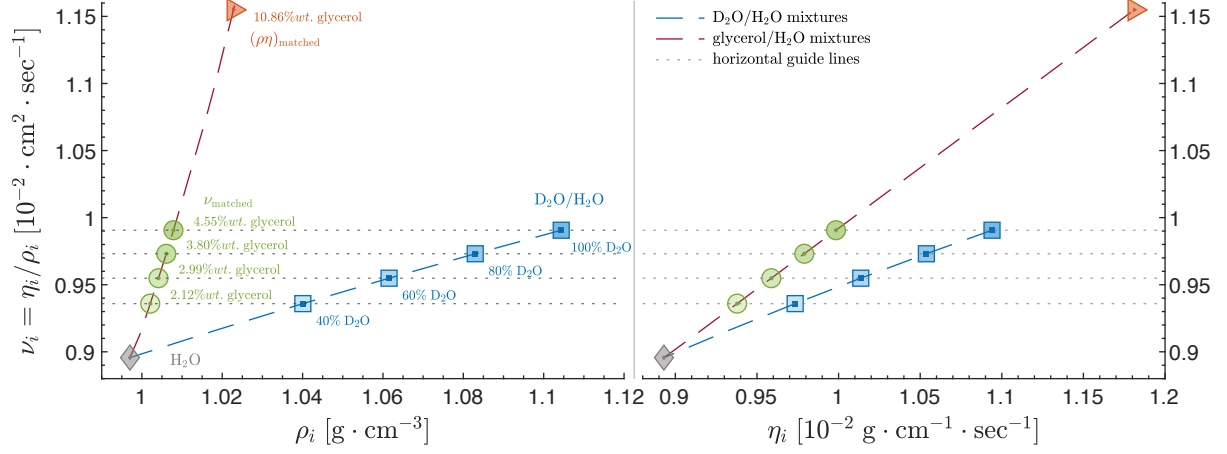

**Figure S1: Physical properties of  $\text{D}_2\text{O}/\text{H}_2\text{O}$  and glycerol/ $\text{H}_2\text{O}$  mixtures at 25 °C.** Kinematic viscosity versus density (left panel) and viscosity (right panel) of  $\text{D}_2\text{O}/\text{H}_2\text{O}$  mixtures and glycerol/ $\text{H}_2\text{O}$  mixtures;  $i$  represents the different solutions. The markers represent  $\text{H}_2\text{O}$  (grey), four different  $\text{D}_2\text{O}/\text{H}_2\text{O}$  mixtures (blue) and four different glycerol/ $\text{H}_2\text{O}$  mixtures which match kinematic viscosity of the  $\text{D}_2\text{O}/\text{H}_2\text{O}$  mixtures (green;  $\nu_{\text{matched}}$ ), and a glycerol/ $\text{H}_2\text{O}$  mixture which match the product of density and dynamic viscosity of 100%  $\text{D}_2\text{O}$  (orange;  $(\rho\eta)_{\text{matched}}$ ). 100%, 80%, 60%, and 40%  $\text{D}_2\text{O}$  correspond to the molar fractions 1.0, 0.8, 0.6, and 0.4 of  $\text{D}_2\text{O}$ .

### S3 Measuring QCM response from different liquids on flat substrates

Fig. S2 shows the experimental procedure for measuring the QCM response from different liquids on flat substrates with the response of the substrate in contact with air as a reference. The experiment starts by establishing a baseline in air, then exchanging to H<sub>2</sub>O until a stable baseline is attained followed by delivering each of the D<sub>2</sub>O/H<sub>2</sub>O and glycerol/H<sub>2</sub>O mixtures for a period of  $\approx 20$  min with an  $\approx 20$  min H<sub>2</sub>O after each step. An extra D<sub>2</sub>O step was added at  $\approx 60$  min to ensure that the signal is stable when the sensor is in contact with D<sub>2</sub>O-containing solutions. The response for each solution was determined by adding the response from exchanging the medium from air to H<sub>2</sub>O,  $\Delta f_{\text{air to H}_2\text{O}}^{\text{substr}}$  or  $\Delta D_{\text{air to H}_2\text{O}}^{\text{substr}}$ , to the response of exchanging the medium from H<sub>2</sub>O to the respective solution, for example in case of D<sub>2</sub>O,  $\Delta f_{\text{H}_2\text{O to D}_2\text{O}}^{\text{substr}}$  or  $\Delta D_{\text{H}_2\text{O to D}_2\text{O}}^{\text{substr}}$ . This approach was applied to minimize errors that could result from signal drift over the long duration of the experiment.

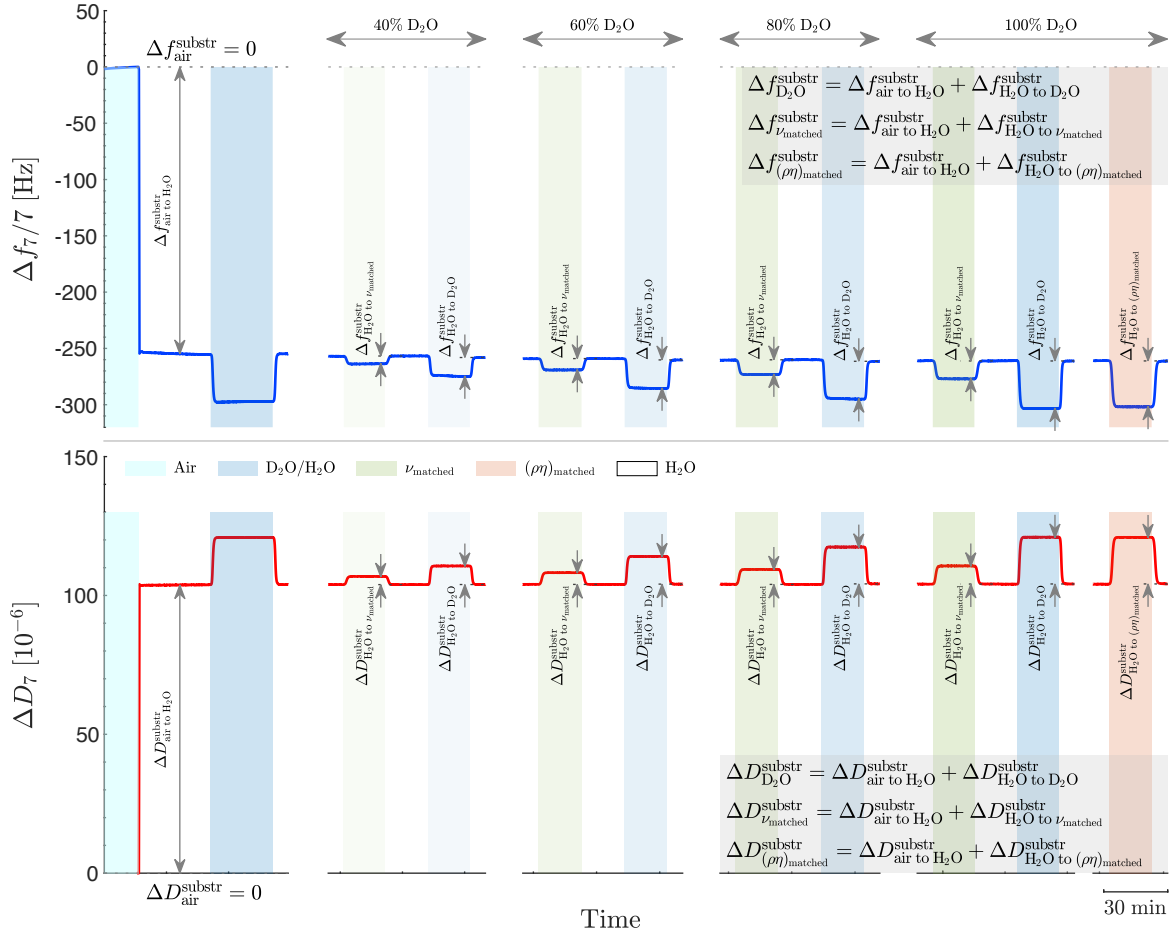

**Figure S2: Experimental procedure to measure the QCM responses on a flat substrate for different solutions with the response of the substrate in contact with air as a reference.** The measured changes in resonance frequency (upper panel) and energy dissipation (lower panel) at the 7<sup>th</sup> overtone versus time. These results were obtained from measurements using an aminated SiO<sub>2</sub>-coated sensor in a citrate-based buffer, pH (pD) = 4.0. The physical properties of all the solutions are given in Table S1.

## S4 QCM response due to adsorption of NPs in different liquids and in air

The experimental procedure for measuring the response in different solutions and in air for adsorption of 150 nm SiO<sub>2</sub> NPs can be summarized in the following steps (Fig. S3):

- (i) establishment of a baseline in air,
- (ii) exchanging to buffers in H<sub>2</sub>O, D<sub>2</sub>O, and a glycerol/H<sub>2</sub>O mixture matching the kinematic viscosity of D<sub>2</sub>O,  $\nu_{\text{matched}}$ ; the responses of these buffers were compared to the theoretically calculated values to verify that there is no major perturbation in system due to air bubbles or any other reason; overtones which showed large deviation from the expected theoretical value were excluded from the calculations,
- (iii) adsorption of PLL to form a positively charged surface,
- (iv) exchanging to D<sub>2</sub>O-based buffer for  $\approx 30$  min to ensure that the signal is stable when the sensor is in contact with D<sub>2</sub>O-containing buffers,
- (v) exchanging to buffers in four different D<sub>2</sub>O/H<sub>2</sub>O mixing ratios and their corresponding buffers in glycerol/H<sub>2</sub>O mixtures matching the kinematic viscosity of the D<sub>2</sub>O/H<sub>2</sub>O mixtures,  $\nu_{\text{matched}}$ ; the D<sub>2</sub>O/H<sub>2</sub>O and glycerol/H<sub>2</sub>O based buffers were delivered for a period of  $\approx 20$  min with an  $\approx 20$  min H<sub>2</sub>O-based buffer after each step,
- (vi) SiO<sub>2</sub> NPs adsorption in H<sub>2</sub>O-based buffer, followed by a NPs-free H<sub>2</sub>O-based buffer,
- (vii) exchanging to 99.7% ethanol for  $\approx 30$  min to account for any changes, e.g., desorption of NPs or spatial reorganization, that would happen in the final drying step under ethanol; this step is followed by H<sub>2</sub>O-based buffer for  $\approx 60$  min,
- (viii) exchanging to D<sub>2</sub>O-based buffer for an  $\approx 30$  min to account for any signal drifts when the sensor is in contact with D<sub>2</sub>O-containing solutions, followed by H<sub>2</sub>O-based buffer for  $\approx 60$  min,
- (ix) exchanging to the same buffers as in step (v) and for similar durations,
- (x) exchanging to 99.7% ethanol before drying the sensor to minimize any drying effects, that would have otherwise affected the response by changing the spatial distribution of the NPs,
- (xi) drying the sensor under N<sub>2</sub> gas while elevating the temperature to 60 °C,
- (xii) lowering the temperature to 25 °C again to measure the response in air,  $\Delta f^{\text{air}}$ , which should be equivalent to response of the dry mass of the adsorbed NPs; a rigorous procedure, as detailed later, was followed to determine if the response in air was really representative of the dry mass of NPs or not.

Note that this lengthy experimental procedure with extra D<sub>2</sub>O and ethanol steps was only required because we wanted to verify the approach at different D<sub>2</sub>O/H<sub>2</sub>O mixing ratios and also to determine the dry mass of the NPs using complementary methods: SEM and QCM in air. For the normal application of the method to determine the dry mass with QCM in a liquid environment, none of these extra steps is needed; it is only required to measure the response in D<sub>2</sub>O and a glycerol/H<sub>2</sub>O mixture matching the kinematic viscosity of D<sub>2</sub>O.

Fig. S4 shows how the response due to the adsorption of NPs was calculated in the different D<sub>2</sub>O/H<sub>2</sub>O and glycerol/H<sub>2</sub>O based buffers; the presented procedure was used to minimize any artifacts that could result from signal drift over the long duration of the experiment. Note that in the superscript NPs, as in  $\Delta f_{\text{H}_2\text{O}}^{\text{NPs}}$  and  $\Delta D_{\text{H}_2\text{O}}^{\text{NPs}}$  in Fig. S4, is only used in the SI and not the main text; this superscript was introduced to differentiate between the substrate, NPs and total responses which are discussed only in the SI as detailed in Section S6.

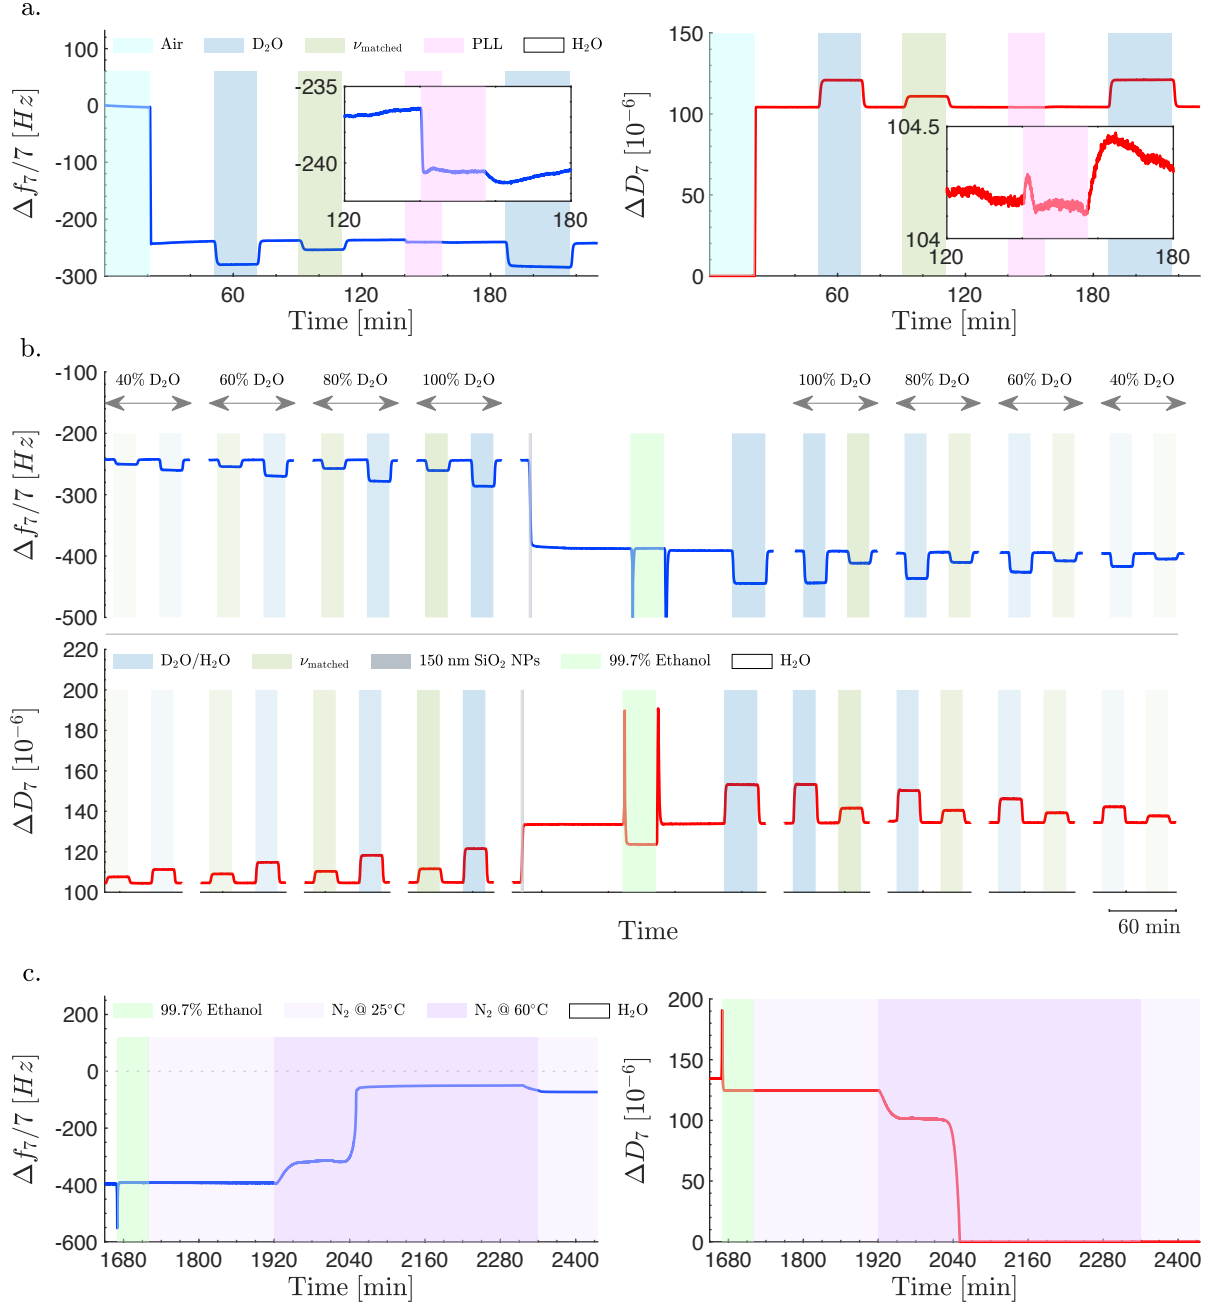

**Figure S3: Experimental procedure to measure and calculate the QCM responses for 150 nm SiO<sub>2</sub> nanoparticles (NPs) adsorption to poly-L-lysine (PLL) in different solutions and in air.** The measured changes in resonance frequency and energy dissipation at the 7<sup>th</sup> overtone for: (a) exchange from air to liquid followed by PLL adlayer formation; (b) SiO<sub>2</sub> NPs adsorption; and (c) drying the sensor under N<sub>2</sub> flow. All solutions contained 10 mM Bis-Tris, pH (pD) = 7, and 150 mM NaCl. The physical properties of all the solutions are tabulated in Table S1.

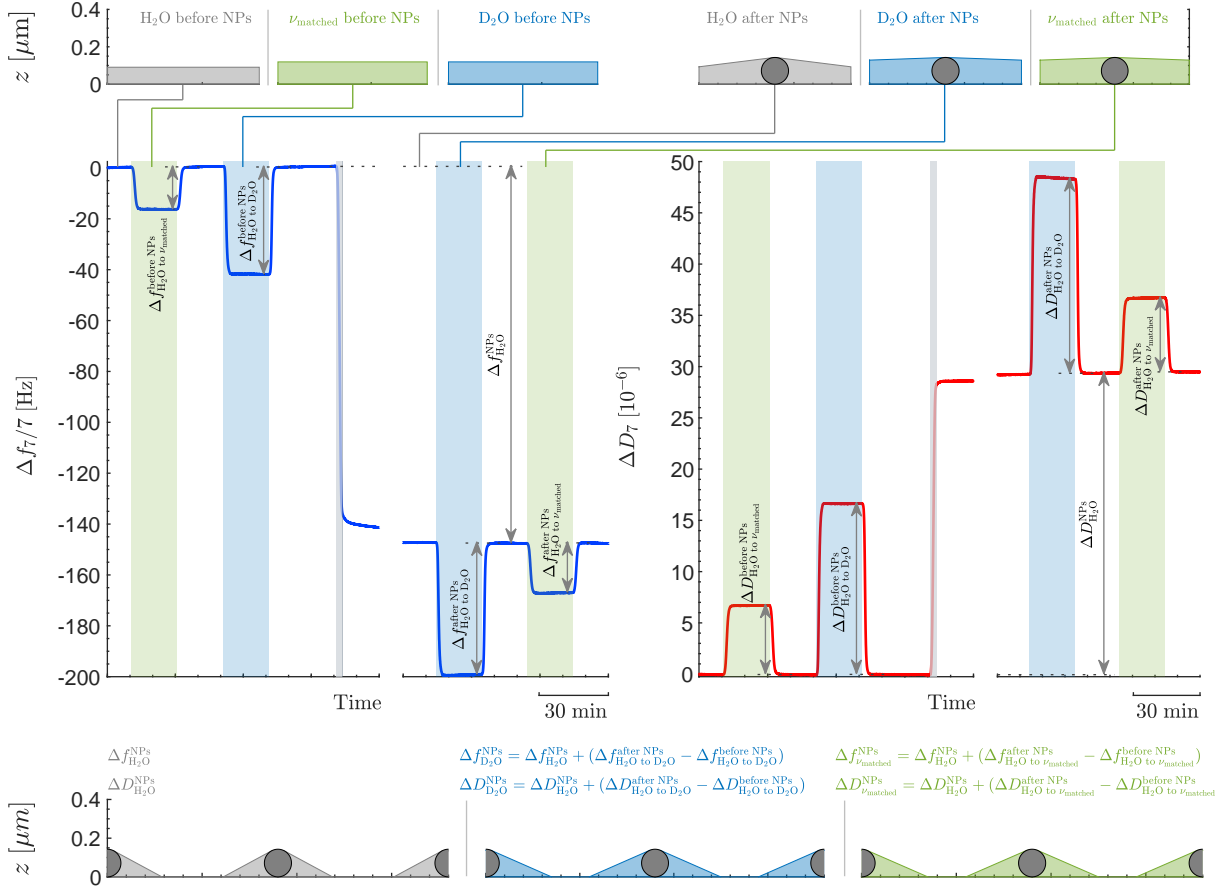

**Figure S4: Experimental procedure to measure the QCM responses for  $\text{SiO}_2$  nanoparticles adsorption in different solutions.** Frequency and dissipation responses versus time for the adsorption of 150 nm  $\text{SiO}_2$  NPs preceded and followed by exchanging the buffer from  $\text{H}_2\text{O}$  to  $\text{D}_2\text{O}$  and  $\nu_{\text{matched}}$ . In principle the response of the NPs in any liquid is the difference between the response in the that liquid after the adsorption of the NPs minus the response in the same liquid before the adsorption of the NPs. The calculation approach shown in the schematic is used to avoid errors that could result from signal drift over the long period of the experiment. The schematics showing the coupled solutions on the bare sensors and in the presence of the NPs are not to scale with magnified differences between the solutions for pedagogical reasons.

## S5 Independent determination of the mass of adsorbed NPs

The dry mass,  $\Delta m^{\text{air/SEM}}$ , of the adsorbed NPs was independently determined using two methods: (i) by utilizing the Sauerbrey equation on the frequency response measured in air at the end of every experiment,  $\Delta m^{\text{air}} = -18 \cdot \Delta f^{\text{air}}$ ; and (ii) by using the surface coverage determined from SEM images of the dried sensor to calculate the dry mass based on NPs size and density of 143 nm (determined using AFM as detailed later in this section) and  $2.0 \pm 0.2 \text{ g} \cdot \text{cm}^{-3}$ , respectively. Both approaches have sources of error and many limitations. The error in the measurement of the QCM in air,  $\Delta f^{\text{air}}$ , was determined by drying three bare sensors (no NPs adsorbed) using the same procedure used for drying the sensors with the adsorbed NPs. The average absolute deviation of  $\Delta f^{\text{air}}$  from 0 plus the standard deviation for these bare sensors was used as the estimated error, which was equal to 9.2 Hz and thus, for all the experiments, the uncertainty in the QCM response in air was presented as  $\Delta f^{\text{air}} \pm 9.2 \text{ Hz}$ . In order to estimate a limit of detection (LOD) and a limit of quantification (LOQ) for  $\Delta f^{\text{air}}$ , we considered the error value of 9.2 Hz to be the standard deviation of the blank (bare sensors),  $S_{\text{blank}}$ . Based on this, we can define the LOD =  $3S_{\text{blank}} = 27.6 \text{ Hz}$  and LOQ =  $10S_{\text{blank}} = 92 \text{ Hz}$  (equivalent to surface coverage,  $\theta \approx 10\%$ ). Using  $\Delta f^{\text{air}}$  as a complementary method comes with the advantage that it measures the mass on the same spatial scale as the QCM measurement in liquid, i.e., over the whole area of the sensor.

Contrary to the  $\Delta f^{\text{air}}$  measurements, the estimations of dry mass based on SEM,  $\Delta m^{\text{SEM}}$ , rely on images that represent only a small portion of the total QCM sensing area and furthermore, require knowledge of both density and size of the NPs. For these reasons, we primarily relied and on  $\Delta f^{\text{air}}$  measurements as an independent control method for determining the dry mass of the adsorbed NPs. However, drying of the sensors was not always successful as is reflected in  $\Delta D^{\text{air}} \gg 0$ , spread out  $\Delta f^{\text{air}}$  from different overtones and/or drying effects, such as NPs aggregation, usually visible with the naked eye. In these cases we thus had to rely on the mass estimation based on the surface coverage obtained from the SEM images, Fig. S5.

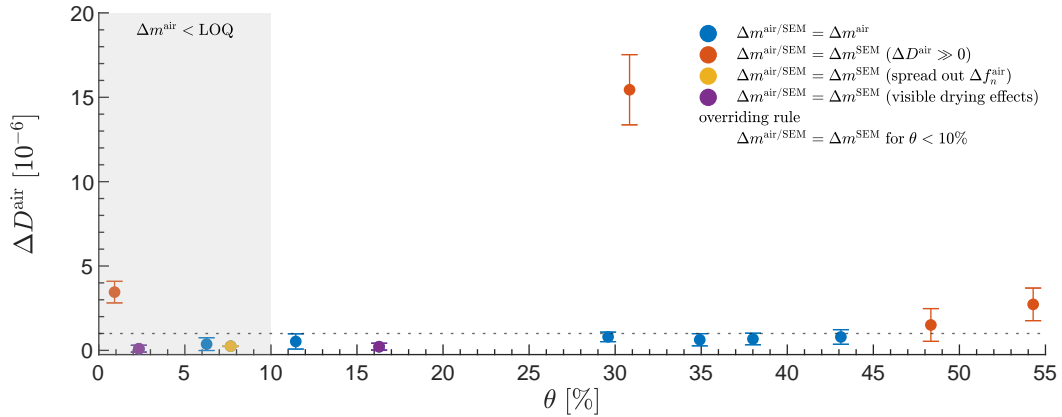

**Figure S5: Molecular mass determination using QCM response in air,  $\Delta m^{\text{air}}$ , or SEM imaging,  $\Delta m^{\text{SEM}}$ .** Average dissipation is plotted versus surface coverage; the dissipation was calculated as an average of 5 different overtones for the measurement in air after drying the sensors. The color coding and legend shows for each experiment which of  $\Delta m^{\text{air}}$  or  $\Delta m^{\text{SEM}}$  was used as a complementary method to determine the dry mass.

In the case of SEM imaging, there are two sources of uncertainty: one relates to uncertainty in coverage estimation and the other to uncertainty in the density of the  $\text{SiO}_2$  NPs, which ranges between 1.8 and  $2.2 \text{ g} \cdot \text{cm}^{-3}$ . Coverage uncertainty varied from one sensor to another, with two major factors affecting the confidence level. The first is drying effects, which resulted in aggregation and redistribution of NPs on the surface, making it challenging to determine the NPs coverage. Drying effects varied from one sensor to another and could be seen both by the naked eye and while imaging. In all the acquired SEM images we stayed as far as possible from the areas where there was clear evidence of drying effects, while simultaneously being as close as possible to the center of the sensor, the region of the sensor which contributes the most to the QCM signal. The second affecting factor is due to inhomogeneous local surface coverages; at high surface coverages, the coverage varied little between different locations, while at low surface coverages the variations in local coverages were substantial. This effect was most pronounced at coverages  $\theta < 10\%$ ,

which is also close to the LOQ for the  $\Delta f^{\text{air}}$ . At this very low surface coverages, we tried to get the best estimate possible using up to 5 images taken at the center of the sensor. Due to these reasons, dry mass estimates using SEM ( $\Delta m^{\text{SEM}}$ ) and QCM in air ( $\Delta m^{\text{air}}$ ) in the low surface coverage regime should be treated qualitatively rather than quantitatively. Finally, some of the acquired images contained features much larger (Fig. S6a) or much smaller (Fig. S6b) than the size of the NPs, which were not included in the estimation of NP surface coverage. However, features which indicated a double layer of NPs (Fig. S6c) were included accordingly.

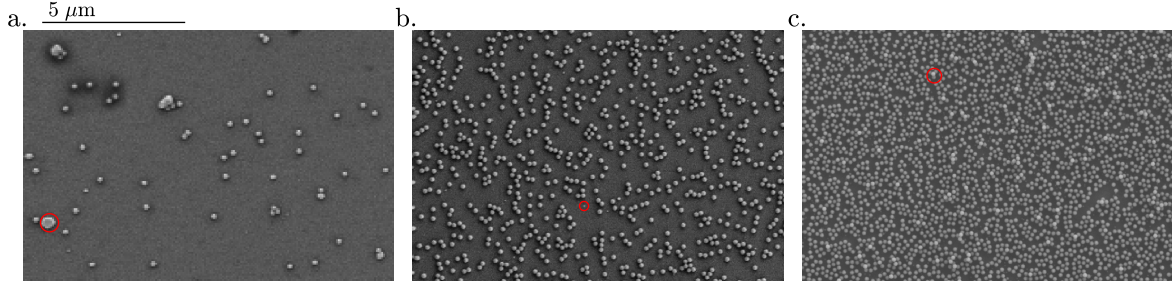

**Figure S6: Counting nanoparticles (NPs) based on SEM images.** The three SEM images show three different sources of artifacts inside the red circles: (a) a feature much larger than the size of NPs, which was not counted; (b) a feature much smaller than the size of NPs, which was not counted; (c) a double layer of NPs which was double counted. The scale bar is  $5 \mu\text{m}$  and applies for all the images.

The following strategy was used with the software imageJ for surface coverage quantification.

1. Crop image to exclude the information bar at the bottom.
2. Set image scaling to correct value based on scale bar of original image.
3. Measure the area of the image.
4. Run Subtract background, rolling ball radius 5 pixels.
5. Copy the cropped image.
6. Apply Gaussian or median filter to copied image (i.e., make sure small features are smoothed).
7. Open set threshold and select Dark Background and Stack histogram and adjust threshold.
8. Run Noise, Remove outliers.
9. Apply math function to divide all pixels by 255 (i.e., make binary).
10. Multiply Binary image with cropped image and run find maxima at minimum prominence ( $> 5\text{-}10$ ).
11. Exclude particles on edges.
12. This procedure will render a value for the number of detected NPs per image.

As noted earlier,  $\Delta m^{\text{SEM}}$  determination requires precise knowledge of the size of the NPs, which was evaluated using AFM. The AFM was conducted using a conventional silicon probe in tapping-mode utilising various drive amplitudes. Multiple images were acquired from one of the dried QCM sensors, all close to the center of the sensor. Images were processed using NanoScope analysis software from Bruker and ImageJ. The following strategy was used for obtaining NP diameter.

1. Open AFM image in NanoScope Analysis software.
2. Perform Plane fit on whole image using a threshold  $< 10 \text{ nm}$ .
3. Save image.
4. Go to Browse files (found to the far right side of the panel) and right click the previously saved image and export as ascii. Select the right number of columns corresponding to the line numbers of the AFM scan.

5. Open the text file and remove the header, save file.
6. Import text file into ImageJ using Import text image.
7. Open histogram and note the modal value of the background (this defines the z-height of the surface).
8. Apply Gaussian filter or similar to flatten out spikes in image.
9. Use ImageJ's find the maxima's, with output maxima with tolerance. This will generate a 8bit thresholded image.
10. Run watershed and then detect particles function to find particles and measure the MAX intensity within each NP.
11. Subtract the background height value (step 7) from each NP max value, which renders the particle diameter.

Fig. S7 shows SEM images for all the conducted experiments, as well as an AFM image and the size distribution used to determine the diameter of the NPs after adsorption.

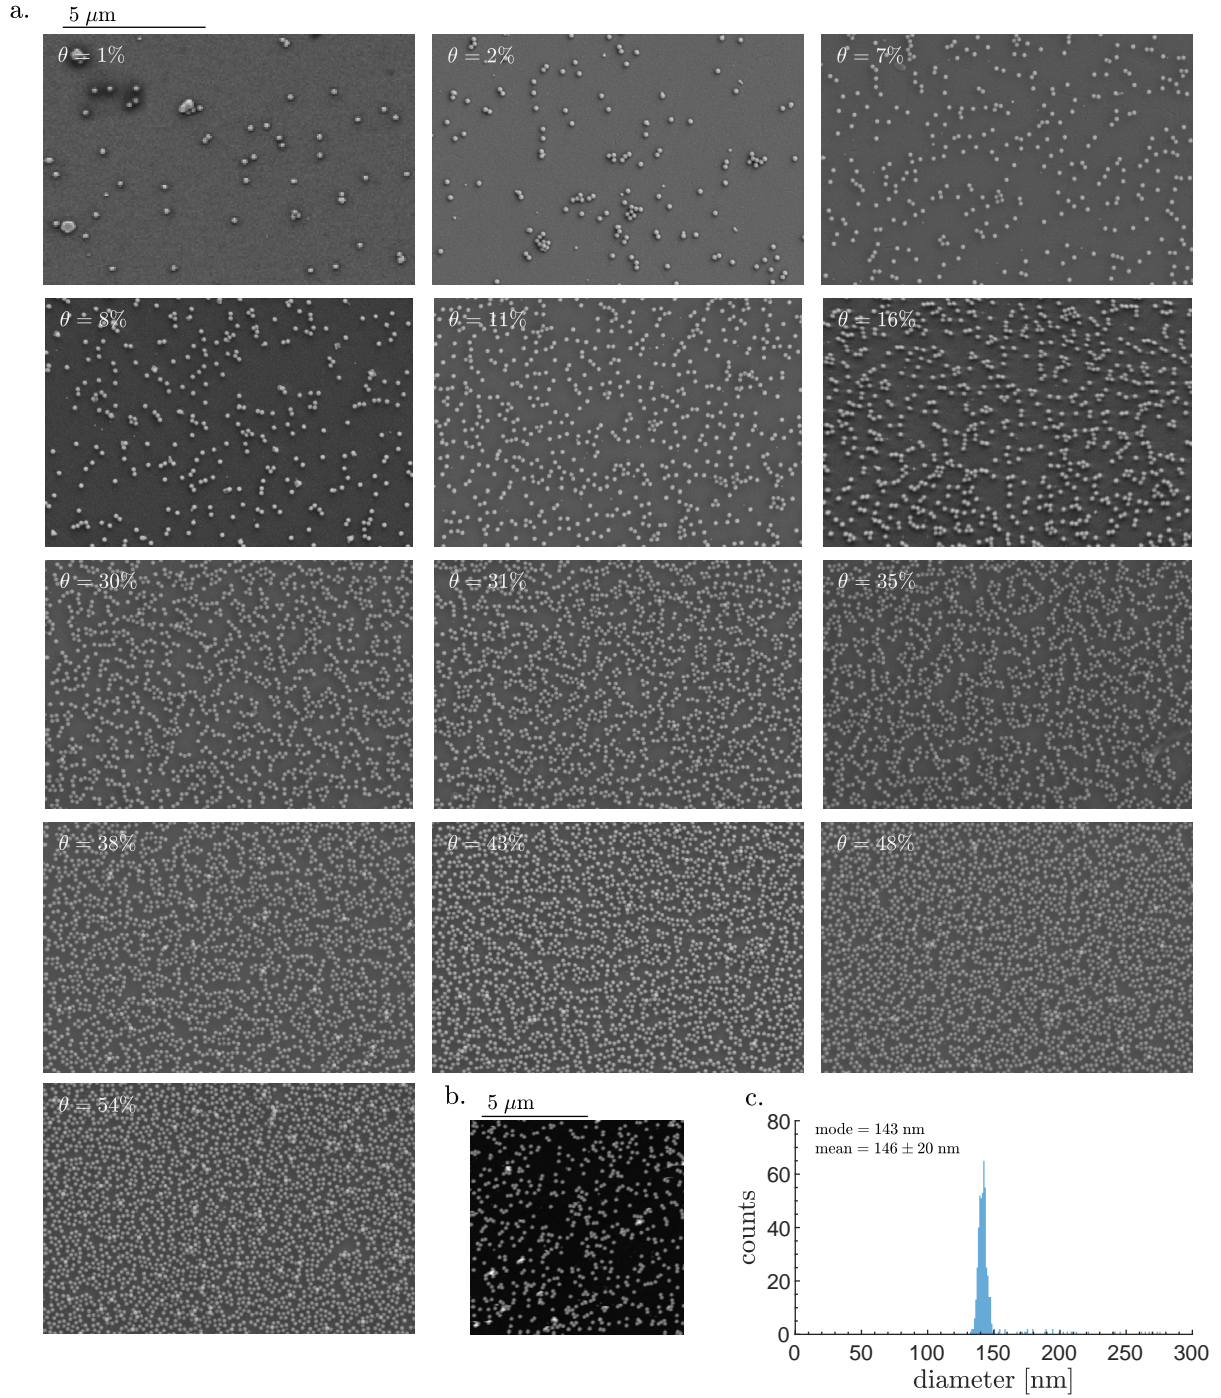

**Figure S7: SEM images at different surface coverages.** (a) SEM images of the adsorbed  $\text{SiO}_2$  NPs on QCM sensors at different surface coverages; the scale bar is  $5\ \mu\text{m}$  and applies for all the images. (b) AFM image of the adsorbed  $\text{SiO}_2$  NPs on a QCM sensor, used to determine the size of the NPs; the scale bar is  $5\ \mu\text{m}$ . (c) Size distribution of  $\text{SiO}_2$  NPs with nominal size of 150 nm and actual size of 143 nm as determined using AFM.

## S6 Theoretical basis for the coupled-liquid response of QCM

In this section, we discuss in more detail Eqs. (2)-(4) presented in the main text. As noticed there, the starting point is the Navier-Stokes equation for the liquid velocity,  $\mathbf{v}$ , [Eq. (15.6) in Ref. 6],

$$\rho \left[ \frac{\partial \mathbf{v}}{\partial t} + (\mathbf{v} \cdot \mathbf{grad}) \mathbf{v} \right] = -\mathbf{grad} p + \eta \nabla^2 \mathbf{v} + \left( \xi + \frac{\eta}{3} \right) \mathbf{grad} \text{div} \mathbf{v}, \quad (\text{S3})$$

where  $\rho$  is the liquid density,  $\eta$  and  $\xi$  are the coefficients of viscosity, and  $p$  is pressure. In application to the QCM measurements, this equation can be simplified by using the following seven points.

(i) Usually, the liquid may be regarded as incompressible, so that  $\text{div} \mathbf{v} = 0$ , and accordingly the last term in Eq. (S3) can be dropped, i.e., we have [Eq. (15.7) in Ref. 6]

$$\frac{\partial \mathbf{v}}{\partial t} + (\mathbf{v} \cdot \mathbf{grad}) \mathbf{v} = -\frac{1}{\rho} \mathbf{grad} p + \nu \nabla^2 \mathbf{v}, \quad (\text{S4})$$

where  $\nu \equiv \eta/\rho$  is the kinematic viscosity.

(ii) The scale of  $\mathbf{v}$  is  $\omega a$ , where  $\omega$  is the QCM frequency, and  $a$  is the amplitude of oscillations of the QCM surface. The scale of the first (linear) term in Eq. (S4) is accordingly given by  $\omega^2 a$ . The scale of the second (quadratic) term in Eq. (S4) is  $\omega^2 a^2/\delta$ , where

$$\delta = (2\nu/\omega)^{1/2} \quad (\text{S5})$$

is the penetration length of QCM oscillations in liquid [Eq. (24.4) in Ref. 6]. Thus, the scale of the ratio of the second and first terms is  $a/\delta$ . For a 5 MHz QCM sensor oscillating at the fundamental tone and immersed in water,  $a$  is a few nm (see e.g., Refs. 7 and 8) and  $\delta \approx 240$  nm, making  $a/\delta$  small, and accordingly the quadratic term in Eq. (S4) can be neglected, i.e.,

$$\frac{\partial \mathbf{v}}{\partial t} = -\frac{1}{\rho} \mathbf{grad} p + \nu \nabla^2 \mathbf{v}. \quad (\text{S6})$$

(iii) The term related to the variation of pressure,  $\mathbf{grad} p$ , can be expressed via the square of the velocity [Eq. (15.11) in Ref. 6] and accordingly can be neglected as well. The validation of this step is similar to that in item (ii). Thus, Eq. (S6) can be reduced to

$$\frac{\partial \mathbf{v}}{\partial t} = \nu \nabla^2 \mathbf{v}. \quad (\text{S7})$$

This equation is identical to Eq. (2) in the main text.

(iv) Many real systems can be described using the equations above with the no-slip boundary condition at the surface- and adsorbate-liquid interfaces, i.e., the condition stating that the liquid velocity at the interface is the same as that of the sensor surface and adsorbate,

$$\mathbf{v}(\mathbf{r})|_{\text{interface}} = \mathbf{v}_{\text{interface}}, \quad (\text{S8})$$

where  $\mathbf{r}$  is the coordinate in the liquid and  $\mathbf{v}_{\text{interface}}$  is the interface velocity. We accept this condition (concerning its applicability, see, e.g. the discussion in Ref. 9). In addition, we will consider that the adsorbate is firmly bound to the QCM surface or its inertia is appreciably larger than that of adjacent liquid, so that the position of the interface is independent of the liquid density.

(v) Eq. (S7) depends only on  $\nu$ , whereas condition (S8) depends only on geometry of the interface, including any adsorbate. Employing Eq. (S7) in combination with condition (S8), we conclude that the solution of Eq. (S7) depends only on  $\nu$  and interfacial geometry.

(vi) The QCM frequency is determined by the equations describing consistently the shear oscillations of the quartz crystal (together with adsorbate) and liquid. The QCM response or, more specifically, the liquid-related change of the QCM frequency,  $\Delta f^{\text{liq}}$ , is proportional to the liquid-related force acting at the surface- and adsorbate-liquid interfaces. This force is proportional to  $\eta$  and the spatial derivative of  $\mathbf{v}$  at the interface along the normal direction [see e.g., the paragraph containing Eq. (24.6) in Ref. 6]. According to item (v), the derivative depends on  $\nu$  and interfacial geometry, and accordingly the force integrated over the interface or  $\Delta f^{\text{liq}}$  can be represented as a product of  $\eta F(\nu)$ , where  $F(\nu)$  is a function dependent on  $\nu$  and interfacial geometry (the former dependence is indicated explicitly). Multiplying and dividing the corresponding expressions by  $\rho$ , taking into account that  $\eta/\rho = \nu$ , and focusing on  $\Delta f^{\text{liq}}$ , we can represent  $\Delta f^{\text{liq}}$  as  $\rho \nu F(\nu)$ , i.e., as a product of  $\rho$  and another function  $[\nu F(\nu)]$ , where the latter depends only on  $\nu$

and interfacial geometry as well. Using  $k_f$  for the designation of the latter function, we have  $\Delta f^{\text{liq}} = k_f \cdot \rho$ . Thus, the measured frequency response,  $\Delta f$ , is given by

$$\Delta f_i = \Delta f^{\text{dry}} + \Delta f_i^{\text{liq}} = \Delta f^{\text{dry}} + k_f \cdot \rho_i, \quad (\text{S9})$$

where  $\Delta f^{\text{dry}}$  is the shift related to the adsorbate under dry conditions [as in Eq. (1) in the main text], and  $i$  is the subscript introduced in order to specify the type of liquid. Eq. (S9) is identical to Eq. (3) in the main text.

(vii) The energy dissipation per unit time in the liquid can be represented as a product of  $\eta$  and the integral (over the space) of the square of the derivative of the velocity with respect to coordinates [Eq. (16.3) in Ref. 6]. According to item (v), this integral depends only on  $\nu$  and interfacial geometry. Thus, the energy dissipation per unit time or  $\Delta D_i^{\text{liq}}$  can be represented as a product of  $\eta$  and a function which depends only on  $\nu$  and interfacial geometry as well. Bearing in mind  $\Delta D_i^{\text{liq}}$  and using  $k_D$  for the designation of this function, we obtain

$$\Delta D_i = \Delta D^{\text{mech}} + \Delta D_i^{\text{liq}} = \Delta D^{\text{mech}} + k_D \cdot \eta_i, \quad (\text{S10})$$

where  $\Delta D^{\text{mech}}$  is the term related to the mechanical stiffness of the attachment between the adsorbate and the substrate surface. Eq. (S10) is identical to Eq. (4) in the main text.

As noticed in the main text, Eqs. (S9) and (S10) are for practical applications nearly useless if experiments are performed with liquid of one type, because the dependence of  $k_f$  and  $k_D$  on  $\nu$  and interfacial geometry is unknown. With exception for the situation of a uniform flat film,  $k_f$  and  $k_D$  can be calculated numerically (see e.g., Refs. 10 and 11; this approach is cumbersome and the corresponding results are not universal) or analytically, but only by employing severe simplifications, e.g., by using Brinkman's mean-field 1D equation for the amplitude of oscillations of the liquid velocity,

$$i\omega v = \eta \frac{d^2 v}{dz^2} + \eta \beta (v_o - v), \quad (\text{S11})$$

as was done in order to describe the liquid-related response of the QCM with a rough surface<sup>12,13</sup> ( $v$  is the liquid velocity along the QCM surface,  $v_o$  is this velocity at the QCM surface,  $z \geq 0$  is the coordinate perpendicular the QCM surface,  $\beta$  is the effective permeability of the nonuniform interfacial layer located at  $0 \leq z \leq L$ , and  $L$  is the thickness of this layer). As declared in the main text, our strategy is different and more general. In particular, we suggest to determine  $k_f$  and  $k_D$  in Eq. (S9) and (S10) and to quantify  $\Delta f^{\text{dry}}$  and  $\Delta D^{\text{mech}}$  experimentally by using liquids matched with respect to their kinematic viscosities, i.e., liquids with identical  $\nu_i$  but different  $\rho_i$  and  $\eta_i$ .

## S7 QCM response with reference to air

In the main text we have shown that extrapolating the QCM response for the adsorption of NPs in  $D_2O$  and  $\nu_{\text{matched}}$  buffers versus  $\rho$  can be used to accurately determine the dry mass of the adsorbate. We here extend on this results and show that the kinematic viscosity matching approach is also equally applicable to measurements taken with the sensor in contact with air as a reference. We also show that additional verification for the approach can be achieved by measuring the response when exchanging the medium in contact with a flat substrate from air to liquid for  $D_2O$  and glycerol/ $H_2O$  mixtures prepared to match the product of  $\rho$  and  $\eta$  of  $D_2O$ , referred to as  $(\rho\eta)_{\text{matched}}$ . The later results, as well as the results obtained for  $\nu_{\text{matched}}$  buffers on flat substrate, can also serve as an internal control for the accuracy of preparation of the matched solutions.

Fig. S8a shows a schematic representing the three measured responses: (i) the response upon replacing the medium in contact with the flat substrate from air to a liquid,  $\Delta f_i^{\text{substr}}$ , (ii) the response induced upon NP adsorption in liquid,  $\Delta f_i^{\text{NPs}}$ , and (iii) the total response after NP adsorption with respect to that in air,  $\Delta f_i^{\text{tot}} (= \Delta f_i^{\text{substr}} + \Delta f_i^{\text{NPs}})$ . Note that in the manuscript,  $\Delta f_i^{\text{NPs}}$  was presented without a superscript, i.e.  $\Delta f_i$ .

Fig. S8b shows the three-step kinematic-viscosity matching procedure in which  $SiO_2$  NPs were electrostatically adsorbed to a smooth poly-L-lysine (PLL)-coated  $SiO_2$  sensor (an extended version of the experiment shown in Figs. 1-2 in the main text). After initial establishment of a baseline in air and injection of buffered  $H_2O$ , the liquid in contact with the surface of the sensor was first replaced with buffered  $D_2O$  followed by buffered  $(\rho\eta)_{\text{matched}}$  and  $\nu_{\text{matched}}$  (step I). This was followed by adsorption of  $SiO_2$  NPs in an  $H_2O$ -based buffer until  $\Delta f$  plateaued (step II), after which the  $(\rho\eta)_{\text{matched}}$ ,  $\nu_{\text{matched}}$  and  $D_2O$  buffers were again subsequently injected into the flow cell (step III). As indicated in Fig. S8b, this procedure enables measurements of  $\Delta f_i^{\text{substr}}$ ,  $\Delta f_i^{\text{NPs}}$ , and  $\Delta f_i^{\text{tot}}$ .

For flat substrates,  $\Delta f_i^{\text{substr}}$  is well known to be proportional to  $(\rho_i\eta_i)^{1/2}$  [see e.g., Eq. (24.6) for the related force in Ref. 6]. This proportionality does not, however, hold for adsorbates with arbitrary shapes. Indeed, as seen in Fig. S8b-c, the frequency responses in  $D_2O$  and  $(\rho\eta)_{\text{matched}}$  are identical for the flat substrates with reference to air, i.e.,  $\Delta f_{D_2O}^{\text{substr}} = \Delta f_{(\rho\eta)_{\text{matched}}}^{\text{substr}}$ , but not after the adsorption of NPs,  $\Delta f_{D_2O}^{\text{NPs}} \neq \Delta f_{(\rho\eta)_{\text{matched}}}^{\text{NPs}}$  and  $\Delta f_{D_2O}^{\text{tot}} \neq \Delta f_{(\rho\eta)_{\text{matched}}}^{\text{tot}}$ . Additionally, a linear extrapolation of the frequency response in  $D_2O$ ,  $\Delta f_{D_2O}^{\text{substr}}$ , and the kinematic-viscosity matched glycerol/ $H_2O$  mixture,  $\Delta f_{\nu_{\text{matched}}}^{\text{substr}}$ , plotted versus  $\rho_i$  (Fig. S8d) yields an intercept at  $\rho = 0$  of  $\Delta f_{\rho=0} = 0$ , being consistent with the fact that there is no adsorption or desorption of material during this step [see Eq. (S9)]. This latter observation provides an internal verification for the accuracy of the preparation of the kinematic viscosity-matched solutions; if the kinematic viscosity was not correctly matched,  $\Delta f_{\rho=0}$  would have not been zero.

The extrapolation of  $\Delta f_{D_2O}^{\text{tot}}$  and  $\Delta f_{\nu_{\text{matched}}}^{\text{tot}}$  resulted in an intercept  $\Delta f_{\rho=0} \approx -530 \text{ Hz}$  ( $\equiv 9540 \text{ ng} \cdot \text{cm}^{-2}$ ) equal to that of the extrapolation of  $f_{D_2O}^{\text{NPs}}$  and  $\Delta f_{\nu_{\text{matched}}}^{\text{NPs}}$ , which is in excellent agreement with the independently determined dry mass of  $10350 \pm 1035 \text{ ng} \cdot \text{cm}^{-2}$ , based on *ex-situ* SEM images obtained after drying the sensor under nitrogen flow (Fig. 1 in the manuscript). These results show that the kinematic matching approach is equally applicable for measurement conducted with reference to liquid or air.

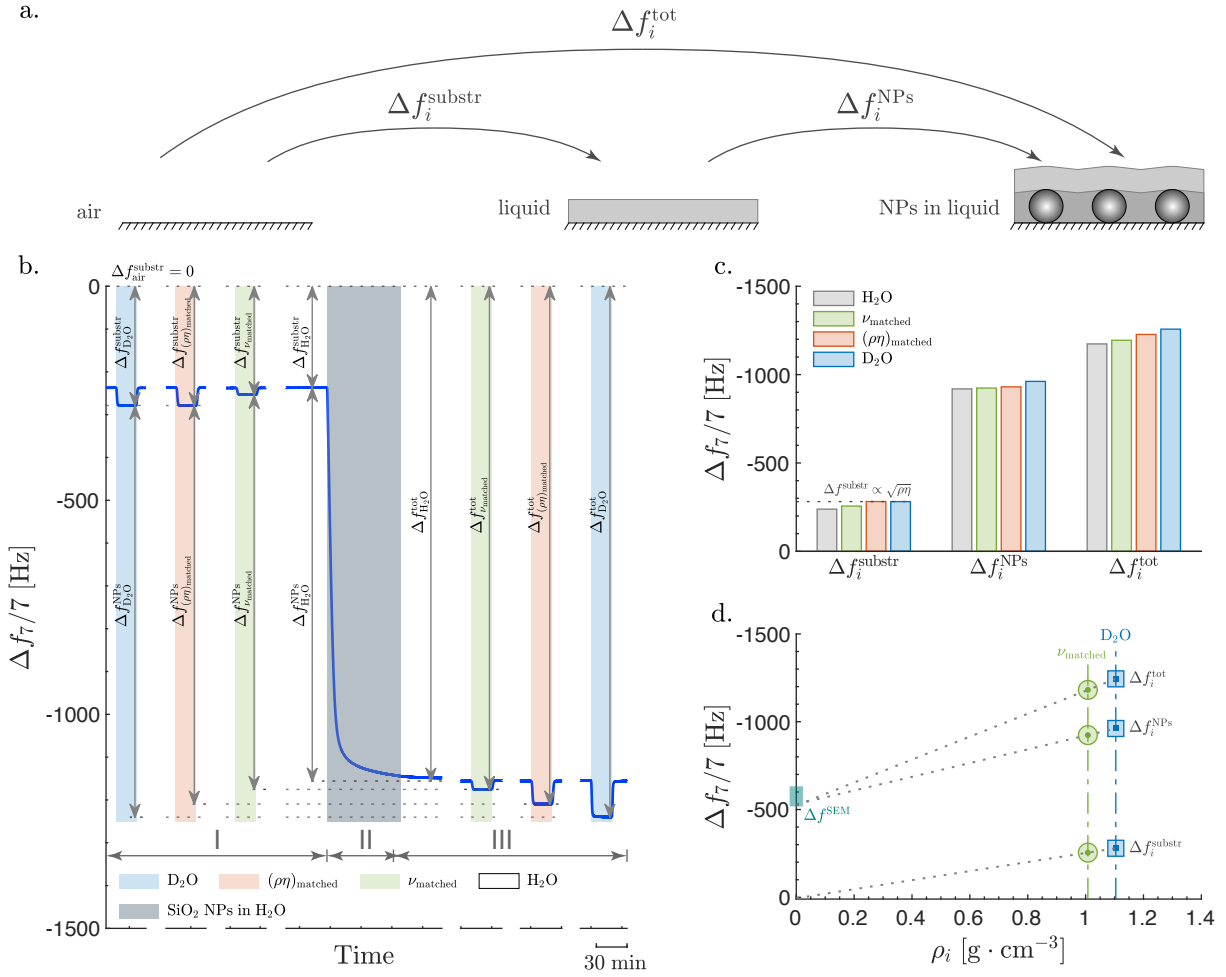

**Figure S8: Experimental procedure for measuring the QCM frequency response in different solutions and disentangling the adsorbate mass and the coupled liquid mass.** (a) A schematic representing the three measured responses: the response upon replacing the medium in contact with the flat substrate from air to a liquid,  $\Delta f_i^{\text{substr}}$ ; the response induced upon NP adsorption in liquid,  $\Delta f_i^{\text{NPs}}$ ; the total response after NP adsorption with respect to that in air,  $\Delta f_i^{\text{tot}} (= \Delta f_i^{\text{substr}} + \Delta f_i^{\text{NPs}})$ . (b) The change in resonance frequency at the 7<sup>th</sup> overtone versus time for (I) a flat substrate in contact with  $\text{H}_2\text{O}$ ,  $\text{D}_2\text{O}$  and glycerol/ $\text{H}_2\text{O}$  mixtures matching the product of the density and viscosity of  $\text{D}_2\text{O}$ ,  $(\rho\eta)_{\text{matched}}$ , and also matching the kinematic viscosity of  $\text{D}_2\text{O}$ ,  $\nu_{\text{matched}}$ ; (II) adsorption of 150 nm  $\text{SiO}_2$  nanoparticles (NPs) on poly-L-lysine (PLL)-coated sensors until the jamming limit (corresponding to a surface coverage of 54%) is reached in an  $\text{H}_2\text{O}$ -based buffer; (III) exchanging the solutions again to  $\nu_{\text{matched}}$ ,  $(\rho\eta)_{\text{matched}}$ , and  $\text{D}_2\text{O}$ . All solutions contained 10 mM Bis-Tris, pH (pD) = 7.0 and 150 mM NaCl. (c) Bar chart showing the different frequency responses:  $\Delta f_i^{\text{substr}}$ ,  $\Delta f_i^{\text{NPs}}$ , and  $\Delta f_i^{\text{tot}}$ , where  $i$  represents four different used solutions:  $\text{H}_2\text{O}$ ,  $\text{D}_2\text{O}$ ,  $(\rho\eta)_{\text{matched}}$ , and  $\nu_{\text{matched}}$ . (d) The different frequency responses in  $\text{D}_2\text{O}$  and  $\nu_{\text{matched}}$  versus liquid density and a linear extrapolation towards vanishing density.  $\Delta f^{\text{SEM}}$  represents the calculated frequency response based on the surface coverage determined using SEM; using a NPs size of 143 nm and density of  $2.0 \pm 0.2 \text{ g} \cdot \text{cm}^{-3}$ . Note that  $\Delta f_i^{\text{substr}}$  plotted in this panel were measured before the PLL adsorption step, and thus are different from the corresponding values shown in panel (b) by  $\approx 4$  Hz.

This analysis of the frequency response with reference to air is equally applicable to the dissipation response. The corresponding changes in  $\Delta D$  are shown in Fig. S9a for the same sequence of injection events shown in Fig. S8b. Similar to the liquid frequency response for flat substrates,  $\Delta D_i^{\text{substr}}$  is well known to be proportional to  $(\rho_i \eta_i)^{1/2}$  [see e.g., Eq. (24.7) in Ref. 6]. As seen in Fig. S9a-b, this proportionality holds for flat substrates with reference to air, i.e.,  $\Delta D_{\text{D}_2\text{O}}^{\text{substr}} = \Delta D_{(\rho\eta)_{\text{matched}}}^{\text{substr}}$ , but not for NPs. Also, similar to the frequency results, extrapolation of  $\Delta D_{\text{D}_2\text{O}}^{\text{substr}}$  and  $\Delta D_{\nu_{\text{matched}}}^{\text{substr}}$ , to  $\eta = 0$  resulted in an intercept  $\Delta D_{\eta=0} \approx 0$ . Finally, the extrapolation of either  $\Delta D_{\text{D}_2\text{O}}^{\text{NPs}}$  and  $\Delta D_{\nu_{\text{matched}}}^{\text{NPs}}$  or  $\Delta D_{\text{D}_2\text{O}}^{\text{tot}}$  and  $\Delta D_{\nu_{\text{matched}}}^{\text{tot}}$  results in almost equal nonzero intercepts of  $\Delta D_{\eta=0} \approx (37 \pm 3) \times 10^{-6}$  at  $\eta = 0$  (Fig. S9c).

All together, these results again verify the generic applicability of the kinematic viscosity matching approach for determination of both  $\Delta f^{\text{dry}}$  and  $\Delta D^{\text{mech}}$  for measurement conducted with reference to either liquid or air.

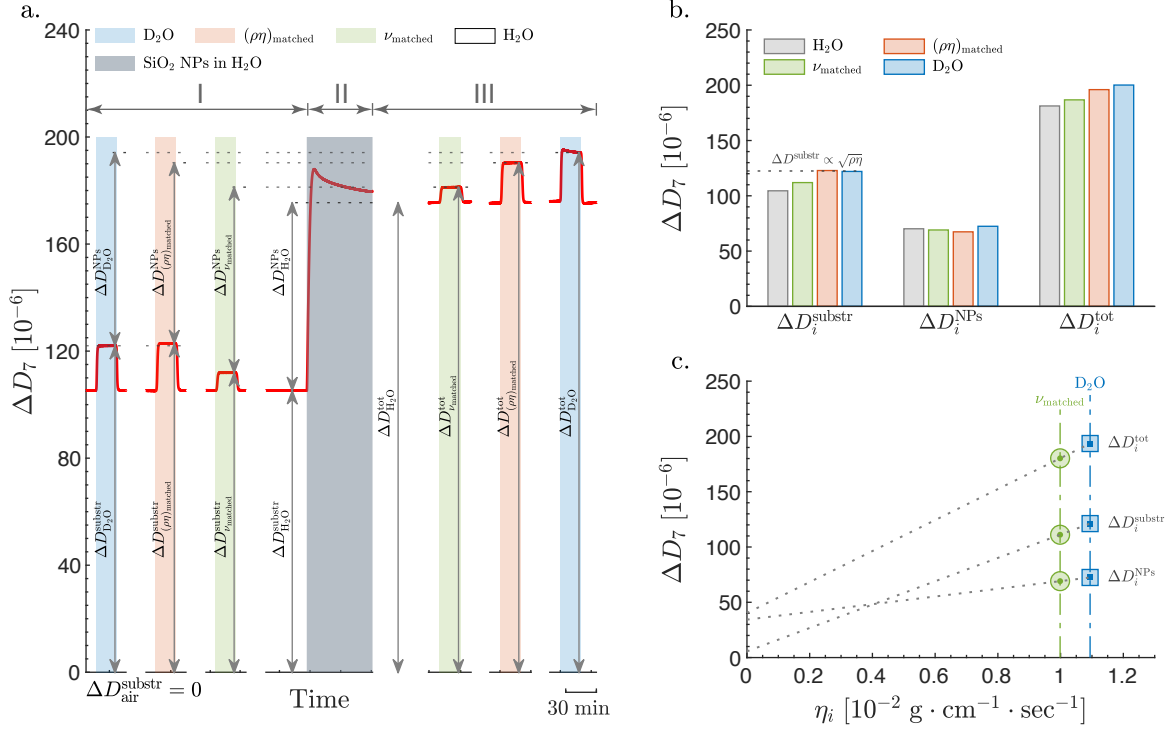

**Figure S9: Experimental procedure for measuring the QCM dissipation response in different solutions and disentangling the mechanical and liquid contributions.** (a) The change in dissipation at the 7<sup>th</sup> overtone versus time for (I) a flat substrate in contact with H<sub>2</sub>O, D<sub>2</sub>O and glycerol/H<sub>2</sub>O mixtures matching the product of the density and viscosity of D<sub>2</sub>O,  $(\rho\eta)_{\text{matched}}$ , and also matching the kinematic viscosity of D<sub>2</sub>O,  $\nu_{\text{matched}}$ ; (II) the adsorption of 150 nm SiO<sub>2</sub> nanoparticles (NPs) on poly-L-lysine (PLL)-coated sensors until the jamming limit is reached in an H<sub>2</sub>O-based buffer; (III) exchanging the solutions again to  $\nu_{\text{matched}}$ ,  $(\rho\eta)_{\text{matched}}$ , and D<sub>2</sub>O. All solutions contained 10 mM Bis-Tris, pH (pD) = 7.0 and 150 mM NaCl. (b) Bar chart showing the responses for:  $\Delta D_i^{\text{substr}}$ ,  $\Delta D_i^{\text{NPs}}$ , and  $\Delta D_i^{\text{tot}}$ , where  $i$  represents four different used solutions: H<sub>2</sub>O, D<sub>2</sub>O,  $(\rho\eta)_{\text{matched}}$ , and  $\nu_{\text{matched}}$ . (c) The different dissipation responses in D<sub>2</sub>O and  $\nu_{\text{matched}}$  versus liquid viscosity and a linear extrapolation towards vanishing viscosity. Note that  $\Delta D_i^{\text{substr}}$  plotted in this panel were measured before the PLL adsorption step, and thus are different from the corresponding values shown in panel (a) by  $\approx 0.1 \times 10^{-6}$ .

To exemplify the uniqueness of the kinematic viscosity matching approach, we compare the extrapolation results from flat substrates to extrapolation using D<sub>2</sub>O with H<sub>2</sub>O and D<sub>2</sub>O with  $(\rho\eta)_{\text{matched}}$  (Fig. S10). The results show that for the extrapolation of the responses in D<sub>2</sub>O with the responses in  $\nu_{\text{matched}}$  buffers resulted in an intercept of  $\Delta f_{\text{D}_2\text{O}/\nu_{\text{matched}}} \approx 0$  and  $\Delta D_{\text{D}_2\text{O}/\nu_{\text{matched}}} \approx 0$ , that was the case for neither the extrapolation of D<sub>2</sub>O with H<sub>2</sub>O buffers ( $\Delta f_{\text{D}_2\text{O}/\text{H}_2\text{O}} \neq 0$  and  $\Delta D_{\text{D}_2\text{O}/\text{H}_2\text{O}} \neq 0$ ) nor for the extrapolation of D<sub>2</sub>O with  $(\rho\eta)_{\text{matched}}$  buffers ( $\Delta f_{\text{D}_2\text{O}/(\rho\eta)_{\text{matched}}} \neq 0$  and  $\Delta D_{\text{D}_2\text{O}/(\rho\eta)_{\text{matched}}} \neq 0$ ).

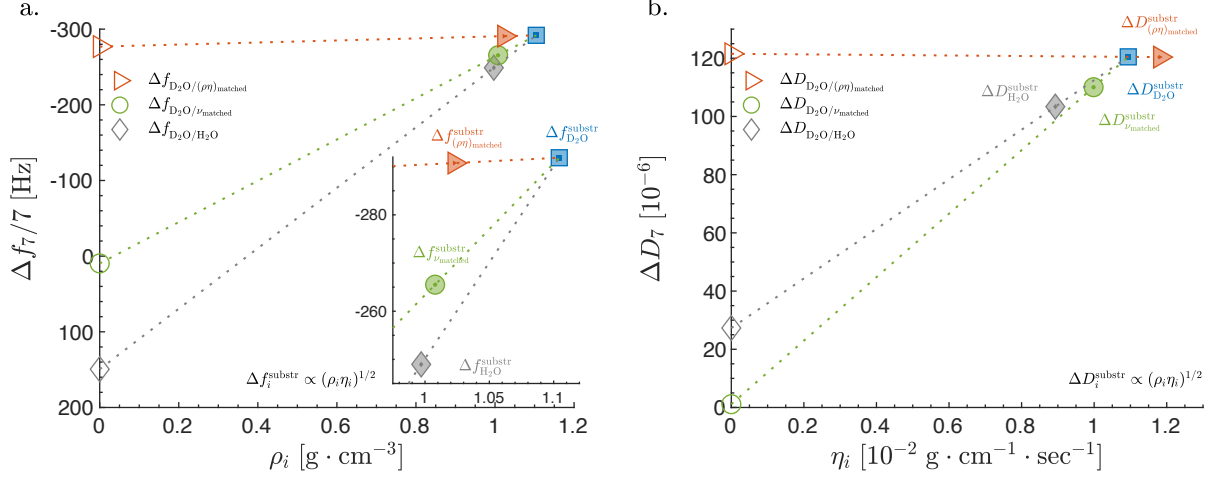

**Figure S10: Liquid contributions to the QCM responses on flat substrates.** (a) Frequency and (b) dissipation responses at the 7<sup>th</sup> overtone plotted versus  $\rho_i$  and  $\eta_i$  for 100% D<sub>2</sub>O, H<sub>2</sub>O,  $\nu_{\text{matched}}$ , and  $(\rho\eta)_{\text{matched}}$  with the frequency and dissipation in air as a reference value, i.e.,  $\Delta f_{\text{air}}^{\text{substr}} = 0$  and  $\Delta D_{\text{air}}^{\text{substr}} = 0$ . Extrapolation lines connecting the 100% D<sub>2</sub>O mixtures with its  $\nu_{\text{matched}}$  (D<sub>2</sub>O/ $\nu_{\text{matched}}$ ) are plotted towards  $\rho = 0$  and  $\eta = 0$ . For comparison, the extrapolation lines connecting 100% D<sub>2</sub>O with H<sub>2</sub>O [D<sub>2</sub>O/H<sub>2</sub>O] and  $(\rho\eta)_{\text{matched}}$  [D<sub>2</sub>O/ $(\rho\eta)_{\text{matched}}$ ] are also shown. All experimental results were obtained from measurements on an aminosilane-modified sensor using citrate-based buffer, pH (pD) = 4.0.

Results for flat substrates have been further verified for different sensors, five different overtones and four different D<sub>2</sub>O/H<sub>2</sub>O mixing ratios (Fig. S11). The results show that for all tested conditions, the extrapolation of the responses in D<sub>2</sub>O/H<sub>2</sub>O mixtures with the responses in their  $\nu_{\text{matched}}$  buffers resulted in an intercept of  $\Delta f_{\text{D}_2\text{O}/\nu_{\text{matched}}} \approx 0$  and  $\Delta D_{\text{D}_2\text{O}/\nu_{\text{matched}}} \approx 0$ , that was not the case when extrapolating D<sub>2</sub>O with H<sub>2</sub>O buffers ( $\Delta f_{\text{D}_2\text{O}/\text{H}_2\text{O}} \neq 0$  and  $\Delta D_{\text{D}_2\text{O}/\text{H}_2\text{O}} \neq 0$ ).

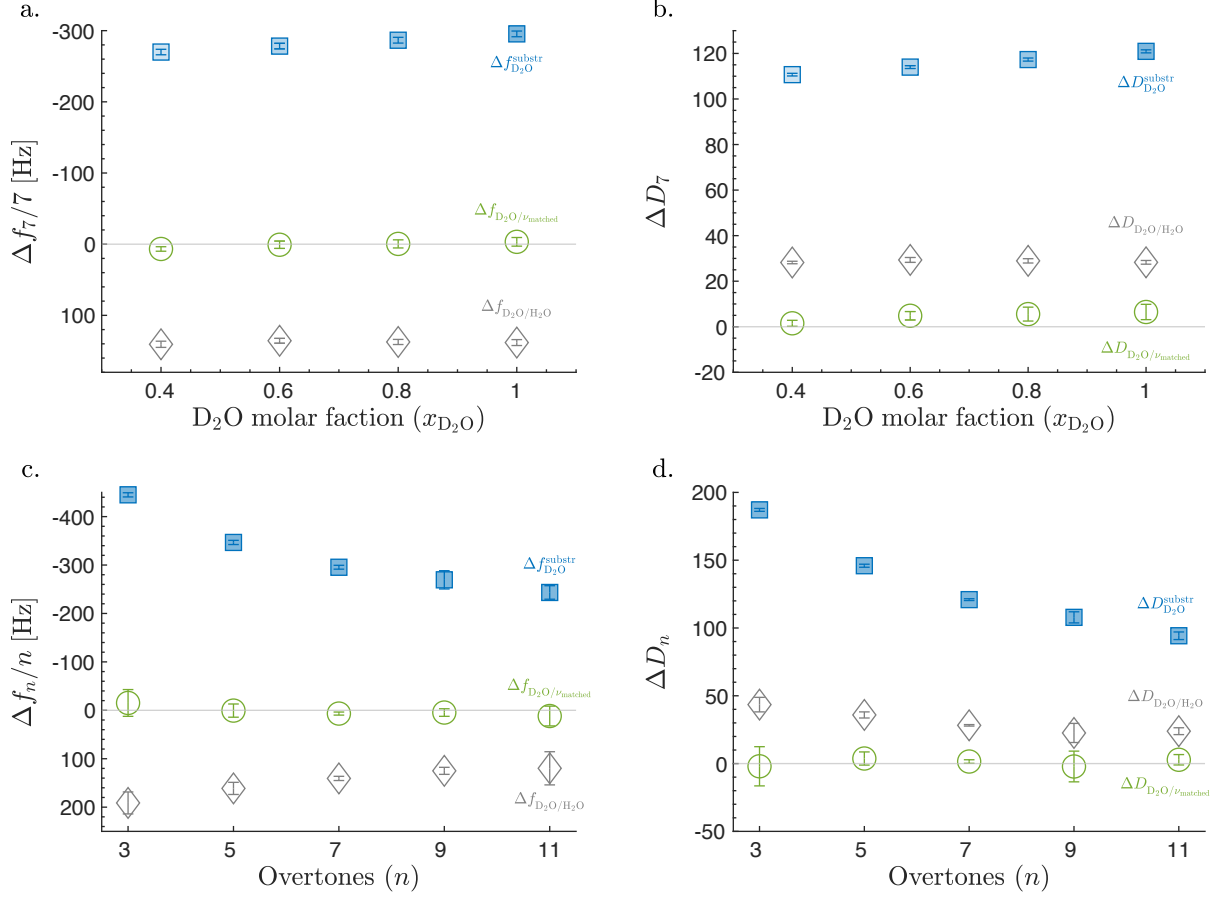

**Figure S11: Liquid contributions to the QCM responses on flat substrates at different D<sub>2</sub>O concentrations and overtones.** (a) Frequency and (b) dissipation responses at the 7<sup>th</sup> overtone plotted versus D<sub>2</sub>O concentration for four different D<sub>2</sub>O/H<sub>2</sub>O mixtures and for the extrapolation with H<sub>2</sub>O [D<sub>2</sub>O/H<sub>2</sub>O] and  $\nu_{\text{matched}}$  [D<sub>2</sub>O/ $\nu_{\text{matched}}$ ] buffers. (c) Frequency and (d) dissipation responses versus the overtone number for 100% D<sub>2</sub>O and for the extrapolation with H<sub>2</sub>O [D<sub>2</sub>O/H<sub>2</sub>O] and  $\nu_{\text{matched}}$  [D<sub>2</sub>O/ $\nu_{\text{matched}}$ ] buffers. The values represent the average of 10 experiments and error bars represent the standard deviation. All experimental results were obtained from measurements on an aminosilane-modified sensor using citrate-based buffer, pH (pD) = 4.0.

## S8 Low charge density of silanized $\text{SiO}_2$ sensors

Fig. S12 shows that both negatively and positively charged polymers adsorb to an aminosilane- (APDMES-) modified surface, even at low salt concentration of 10 mM, i.e., at long ranged Debye length, suggesting a low charge density and thus weak electrostatic interactions for the APDMES-modified surfaces.

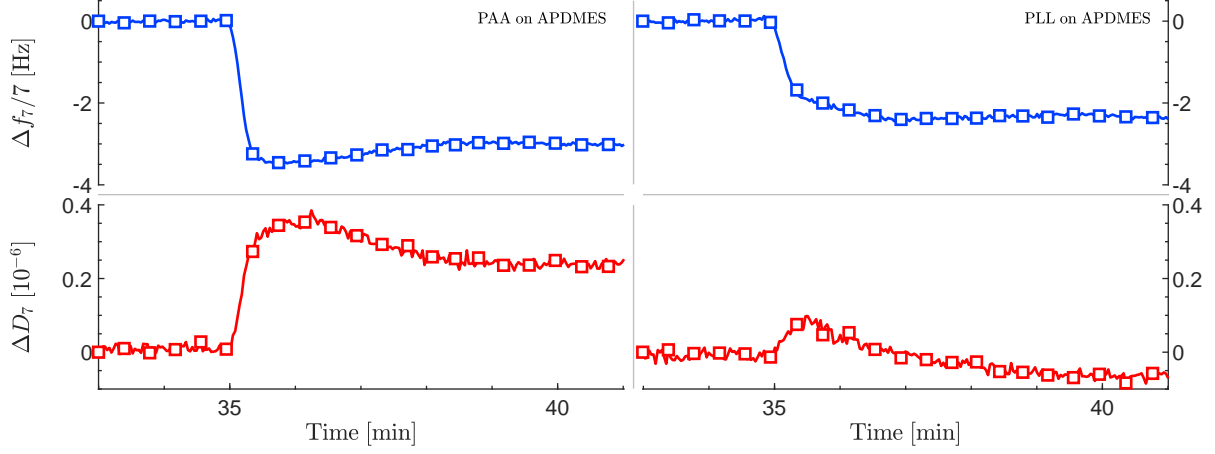

**Figure S12: Adsorption of negatively and positively charged polymers to aminosilane-modified sensors.** Frequency (upper panels) and dissipation (lower panels) changes as a function of time for the adsorption of a negatively charged polymer (poly(acrylic acid); PAA) and a positively charged polymer (poly-L-lysine; PLL) on  $\text{SiO}_2$  sensors modified with amine-terminated silanes (APDMES). Both polymers adsorbed to the surface suggesting a low charge density of the APDMES. All experiments were conducted in a 3 mM Bis-Tris Buffer, pH = 7.0, and total ionic strength  $I = 10$  mM adjusted using NaCl.

## S9 Effect of D<sub>2</sub>O concentration on the measured and extrapolated responses

Fig. S13 shows the frequency,  $\Delta f_{\rho=0}$ , and dissipation,  $\Delta D_{\eta=0}$ , obtained by extrapolation of the response in four different D<sub>2</sub>O/H<sub>2</sub>O mixtures with their corresponding kinematic viscosity matched glycerol/H<sub>2</sub>O mixtures to  $\rho = 0$  and  $\eta = 0$ . Both  $\Delta f_{\rho=0}$  and  $\Delta D_{\eta=0}$  seem to be independent of the D<sub>2</sub>O concentration. Such results provide additional verification for the kinematic viscosity matching approach to determine the adsorbate mass and the mechanical properties of the adsorbate/surface interactions. This additional evidence was not necessary for the verification of the accuracy of  $\Delta f_{\rho=0}$  to determine the adsorbate mass, because enough evidence has already been provided based on the results from QCM in air and SEM imaging. It is, however, more important in the case of  $\Delta D_{\eta=0}$ , because there is little known about the nature of the mechanically dissipated energy and whether it is affected by the properties of the solution. These results suggest that the mechanically dissipated energy was not affected by the different liquid properties within the range of liquids used in this work. If there were a dependency on the liquid properties one would have expected a systematic increase or decrease in  $\Delta D_{\eta=0}$  with the increasing D<sub>2</sub>O concentrations in the D<sub>2</sub>O/H<sub>2</sub>O mixtures.

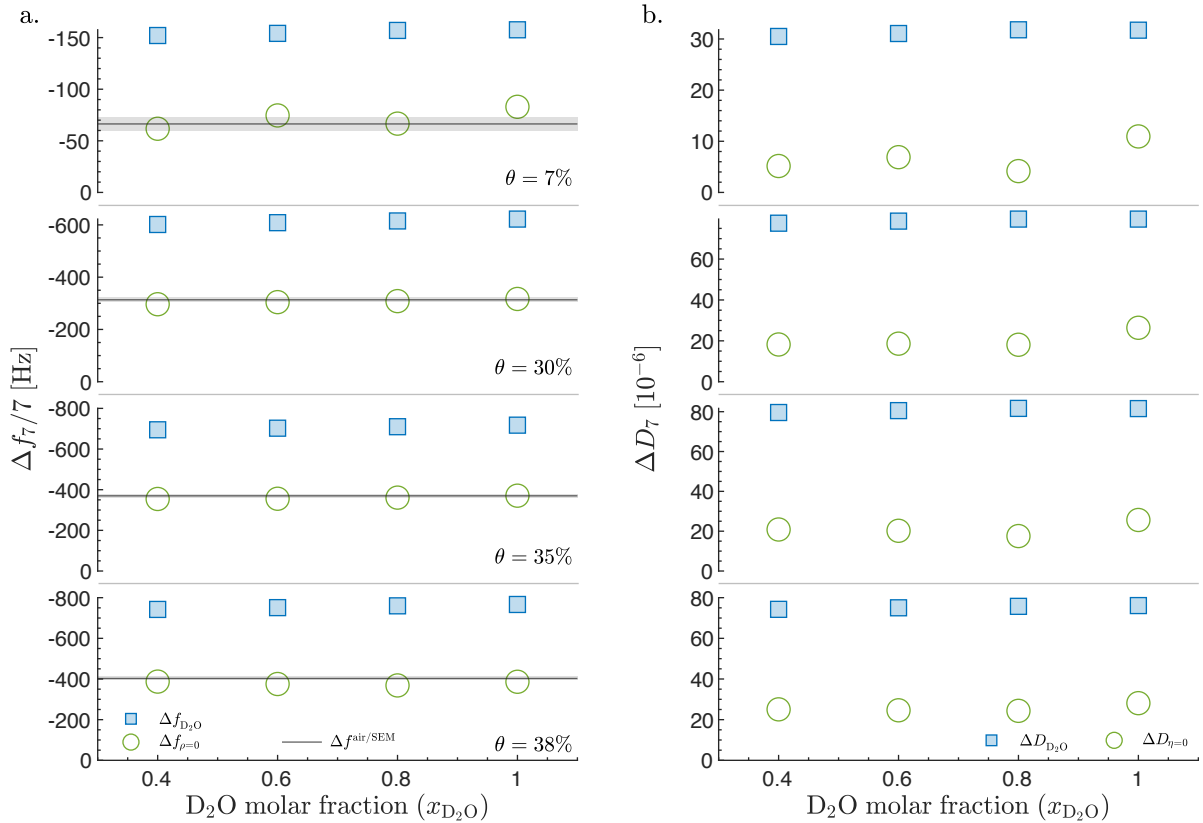

**Figure S13: The dependence of the measured and extrapolated QCM response from adsorbed SiO<sub>2</sub> nanoparticles (NPs) on D<sub>2</sub>O/H<sub>2</sub>O mixing ratios.** (a) Measured frequency shift in four different D<sub>2</sub>O/H<sub>2</sub>O mixtures,  $\Delta f_{D_2O}$ , and extrapolated frequency shift,  $\Delta f_{\rho=0}$ , versus D<sub>2</sub>O concentration,  $x_{D_2O}$ , for adsorption of 150 nm SiO<sub>2</sub> NPs at different surface coverages,  $\theta$ . Shown as well is the frequency shift determined using QCM in air or SEM,  $\Delta f^{air/SEM}$ , with the shaded area representing the uncertainty in  $\Delta f^{air/SEM}$ . (b) Measured dissipation in four different D<sub>2</sub>O/H<sub>2</sub>O mixtures,  $\Delta D_{D_2O}$ , and extrapolated dissipation,  $\Delta D_{\eta=0}$ , versus D<sub>2</sub>O concentration,  $x_{D_2O}$ , for the adsorption of 150 nm SiO<sub>2</sub> NPs at different  $\theta$ . All solutions contained 10 mM Bis-Tris, pH (pD) = 7.0 and 150 mM NaCl.

## S10 Effect of the overtone number on the measured and extrapolated responses

Fig. S14 shows a schematic demonstrating how the increase in overtone number at different surface coverages affects both the liquid frequency response,  $\Delta f^{\text{liq}}$ , and the mechanically dissipated energy per dry mass, represented as  $\Delta D_{\eta=0}/\Delta f_{\rho=0}$ . As  $n$  increases, i.e., as the frequency of oscillation increases, the liquid frequency response,  $\Delta f^{\text{liq}}$ , decreases (Fig. S15) and the mechanical dissipation per dry mass,  $\Delta D_{\eta=0}/\Delta f_{\rho=0}$ , increases (Fig. S16). These effects are dependent on surface coverage,  $\theta$ , with stronger overtone-dependence for  $\Delta f^{\text{liq}}$  at lower surface coverages.

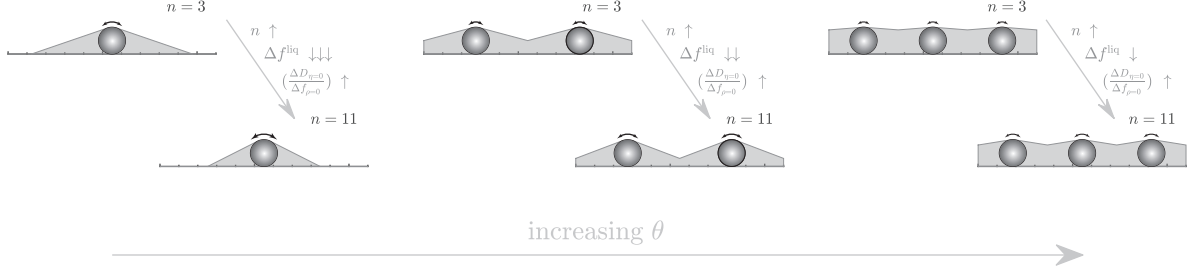

**Figure S14: Overtone dependence of the QCM response for adsorption of spherical nanoparticles (NPs).** A schematic illustrating the change in the liquid frequency response,  $\Delta f^{\text{liq}}$ , and the mechanically dissipated energy per dry mass, represented as  $\Delta D_{\eta=0}/\Delta f_{\rho=0}$ , with overtone number,  $n$ , at different surface coverages,  $\theta$ .

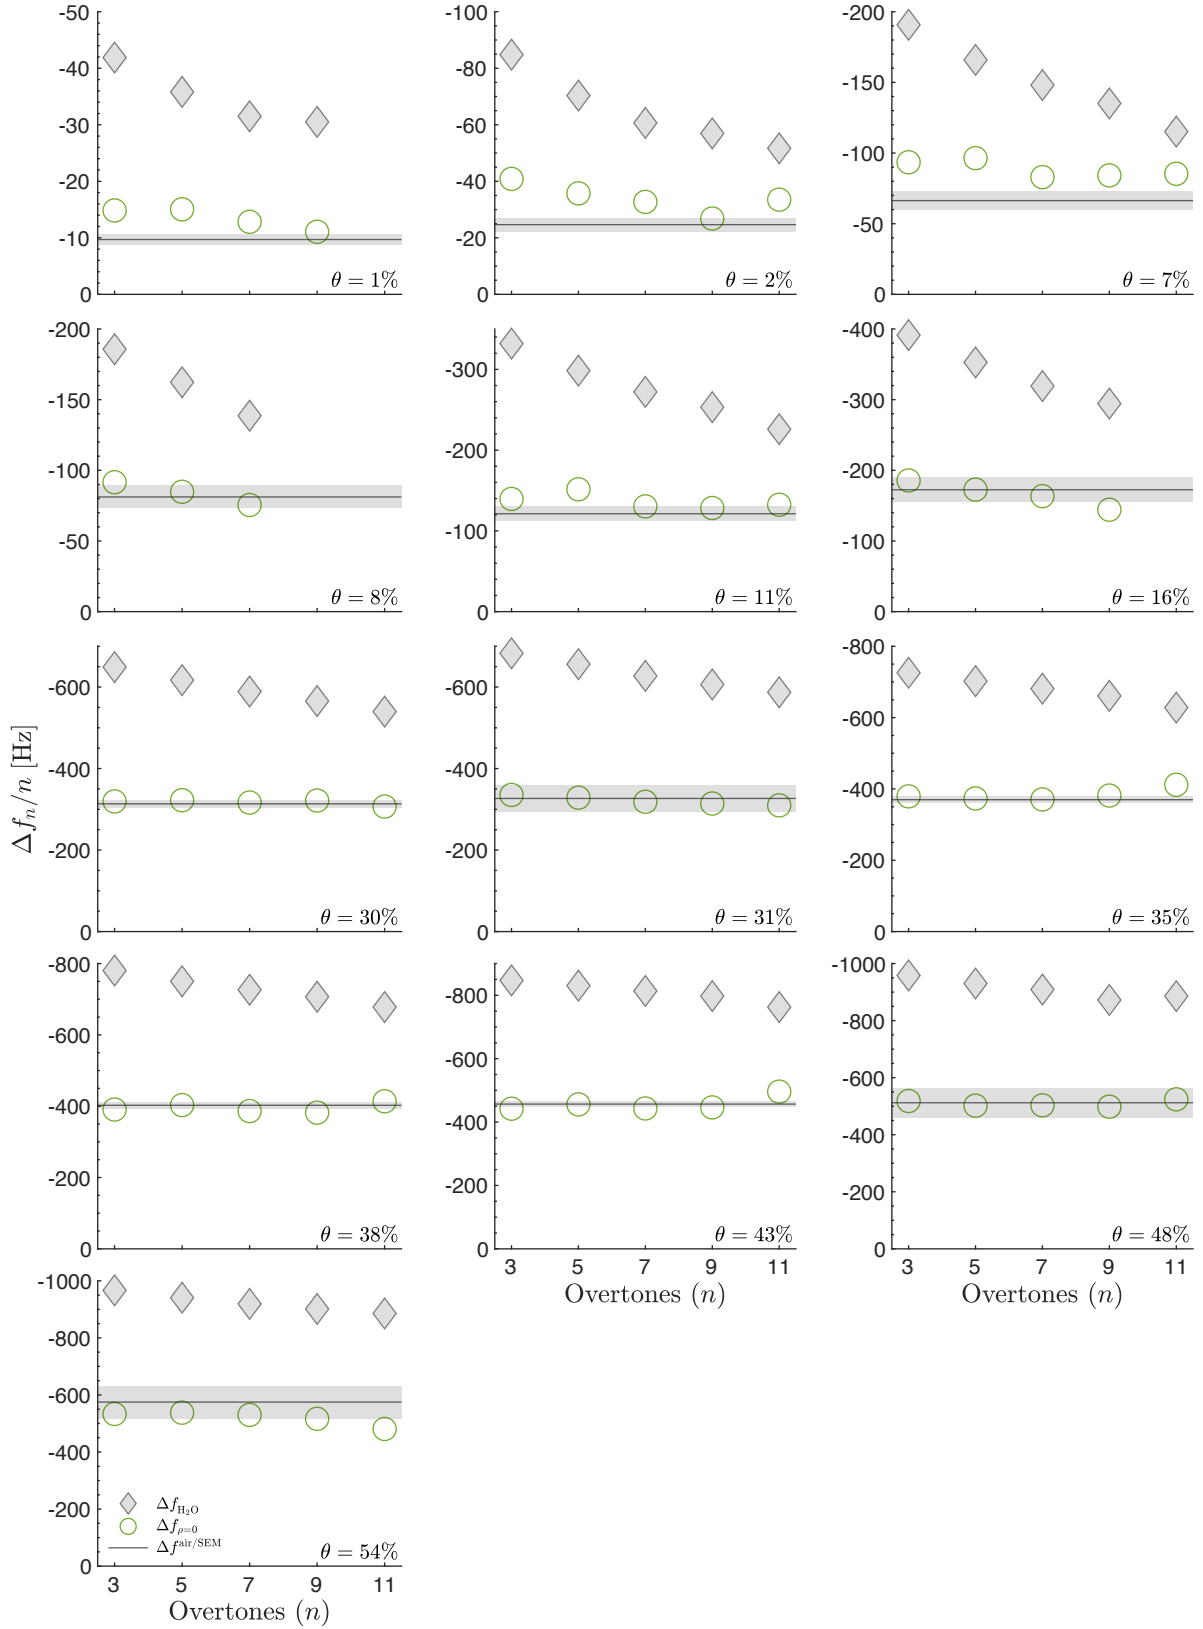

**Figure S15: The dependence of the measured and extrapolated QCM frequency response from adsorbed SiO<sub>2</sub> nanoparticles (NPs) on the overtone number.** Measured frequency shift in H<sub>2</sub>O,  $\Delta f_{\text{H}_2\text{O}}$ , and extrapolated frequency shift,  $\Delta f_{\rho=0}$ , versus the overtone number for adsorption of 150 nm SiO<sub>2</sub> NPs at different surface coverages,  $\theta$ . Shown as well is the frequency shift determined using QCM in air or SEM,  $\Delta f^{\text{air/SEM}}$ , with the shaded area representing the uncertainty in  $\Delta f^{\text{air/SEM}}$ . All solutions contained 10 mM Bis-Tris, pH (pD) = 7.0 and 150 mM NaCl.

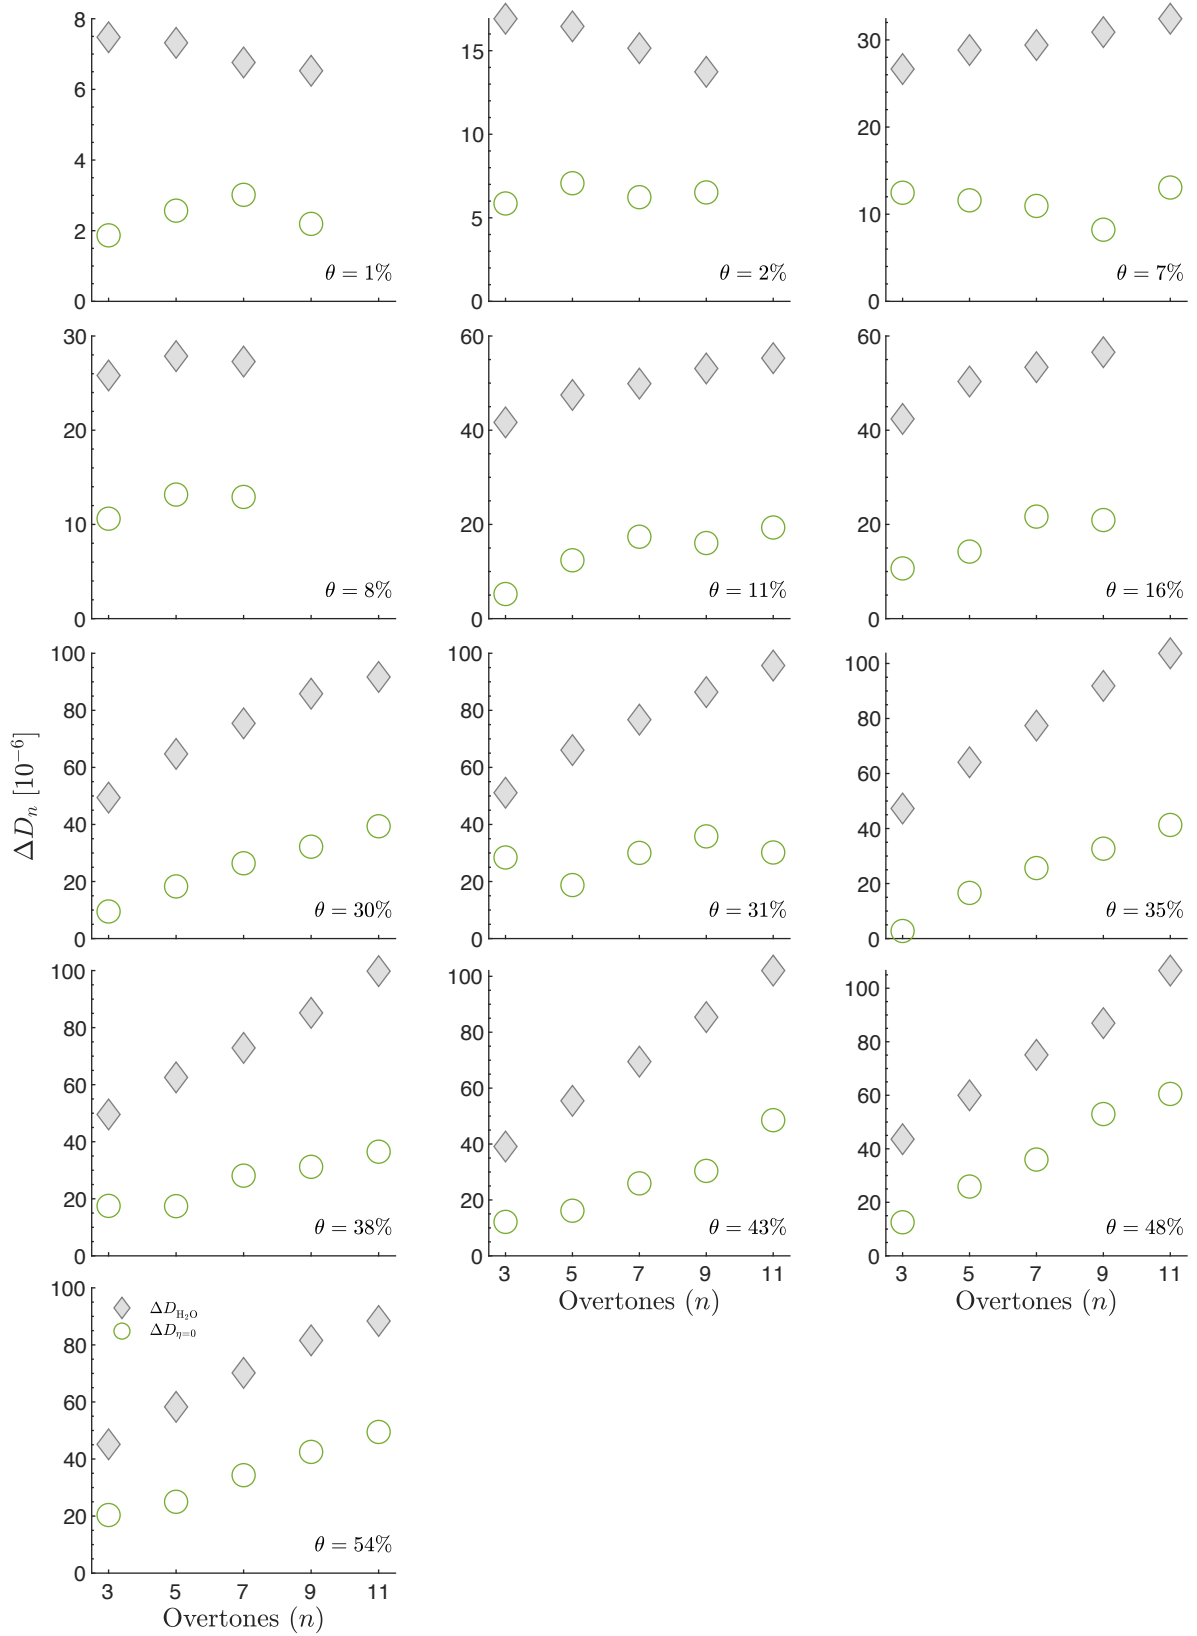

**Figure S16: The dependence of the measured and extrapolated QCM dissipation response from adsorbed SiO<sub>2</sub> nanoparticles (NPs) on the overtone number.** Measured dissipation in H<sub>2</sub>O,  $\Delta D_{H_2O}$ , and extrapolated dissipation,  $\Delta D_{\eta=0}$ , versus the overtone number for adsorption of 150 nm SiO<sub>2</sub> NPs at different surface coverages,  $\theta$ . All solutions contained 10 mM Bis-Tris, pH (pD) = 7.0 and 150 mM NaCl.

## S11 Surface plasmon resonance results for humic acids adlayer

Fig. S17 shows the change in the angle representing surface plasmon resonance,  $\Delta R_\lambda$ , for two wavelengths,  $\lambda = 680$  and  $785$  nm, upon adsorption of PLL followed by humic acids adsorption on a silica-coated sensor. If the refractive index increment,  $dn/dc$ , and the thickness of the adsorbate,  $d$ , are known, the dry mass can be calculated as follows<sup>14, 15</sup>

$$\Delta m^{\text{SPR}} = \frac{d}{S(dn/dc)[1 - \exp(-2d/\delta)]} \cdot \Delta R_\lambda \quad (\text{S12})$$

where  $S$  is the sensitivity in  $^\circ/\text{RIU}$  and  $\delta$  is the decay length of the SPR evanescent field. The sensitivity,  $S$ , was determined for similar silica-coated sensors by measuring the response upon exchanging the liquid in contact with the sensors from  $\text{H}_2\text{O}$  to  $\text{D}_2\text{O}$ ;  $S$  was found to be 112 and  $97^\circ/\text{RIU}$  at  $\lambda = 670$  and  $785$  nm, respectively.

Theoretical determination of the decay length,  $\delta$ , requires knowledge about the thicknesses of all the layers forming the sensor, i.e., Cr, Au, and  $\text{SiO}_2$ . The thicknesses of Cr and Au were assumed to be 1 and 50 nm, respectively, based on the manufacturer's estimation. To determine the thickness of the  $\text{SiO}_2$  coating, the metal surface (1 nm Cr + 50 nm Au) was first modelled by Fresnel equations as described previously<sup>16</sup>. Next, the model was extended to include an additional film with refractive index 1.4628, representing the refractive index of  $\text{SiO}_2$  at  $\lambda = 670$  nm. The thickness of this layer that best matched experimental data was determined to be 15 nm. To estimate the decay length in a water environment, the  $\text{SiO}_2$ -coated SPR model was extended to include an additional layer with refractive index of 1.34, which is slightly above that of a water environment (1.33). This created a clear shift in the simulations while still keeping the effective refractive index of the environment close to water. The simulated SPR angle shift obtained was plotted against the film thickness,  $d$ . This curve was then fitted to a model  $A \cdot [1 - \exp(-2d/\delta)]$  and the  $\delta$  parameter was extracted as the field decay parameter. The fit to the simulated shifts was always excellent with  $R^2 > 0.99$ . These calculations yielded  $\delta = 202$  and  $290$  nm for  $\lambda = 670$  and  $785$  nm, respectively.

The thickness of the HA adlayer,  $d$ , was estimated to be  $\approx 18$  nm based on the ratio of the response at different wavelengths,  $\Delta R_{670 \text{ nm}}/\Delta R_{785 \text{ nm}}$ .<sup>17</sup>

Using  $0.28 \text{ cm}^3 \cdot \text{g}^{-1}$  for the  $dn/dc$  of HA<sup>18</sup>, we obtain  $\Delta m^{\text{SPR}} = 535$  and  $506 \text{ ng} \cdot \text{cm}^{-2}$  at  $\lambda = 670$  and  $785$  nm, respectively, which is in strikingly good agreement with the dry mass of  $535 \pm 40 \text{ ng} \cdot \text{cm}^{-2}$  determined using the kinematic viscosity approach (Fig. 5 in main text).

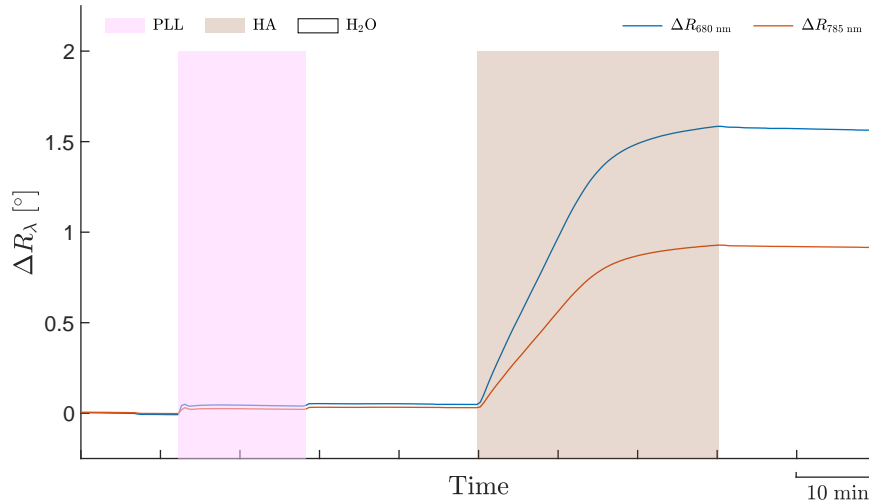

**Figure S17: Surface plasmon resonance (SPR) results for humic acids (HA) adlayer.** The change in the angle of surface plasmon resonance,  $\Delta R_\lambda$ , at two wavelengths,  $\lambda = 680$  and  $785$  nm, due to adsorption of PLL followed by HA on a silica-coated sensor. All solutions contained 10 mM Bis-Tris, pH = 7.0, 150 mM NaCl and 2.5 mM  $\text{CaCl}_2$ .

## References

- [1] J. Kestin, N. Imaishi, S.H. Nott, J.C. Nieuwoudt, and J.V. Sengers. Viscosity of light and heavy water and their mixtures. *Physica A: Statistical Mechanics and its Applications*, 134(1):38–58, 1985.
- [2] M. Nakamura, K. Tamura, and S. Murakami. Isotope effects on thermodynamic properties: mixtures of  $x(\text{D}_2\text{O or H}_2\text{O}) + (1 - x)\text{CH}_3\text{CN}$  at 298.15 K. *Thermochimica Acta*, 253:127–136, 1995.
- [3] M. L. Sheely. Glycerol viscosity tables. *Industrial & Engineering Chemistry*, 24(9):1060–1064, 1932.
- [4] Glycerine Producers’ Association. *Physical properties of glycerine and its solutions*. Glycerine Producers’ Association, New York, 1963.
- [5] JR Cooper and RB Dooley. The international association for the properties of water and steam. *Revised Release on Viscosity and Thermal Conductivity of Heavy Water Substance*, 2007.
- [6] L.D. Landau and E.M. Lifshitz. Viscous Fluids. In *Fluid Mechanics*, chapter 14, pages 44–94. Pergamon Press, 1987.
- [7] M. Edvardsson, M. Rodahl, B. Kasemo, and F. Höök. A dual-frequency QCM-D setup operating at elevated oscillation amplitudes. *Analytical Chemistry*, 77(15):4918–4926, 2005.
- [8] M. Edvardsson, V. P. Zhdanov, and F. Höök. Controlled radial distribution of nanoscale vesicles during binding to an oscillating QCM surface. *Small*, 3(4):585–589, 2007.
- [9] V. P. Zhdanov. How the partial-slip boundary condition can influence the interpretation of the DLS and NTA data. *Journal of Biological Physics*, pages 169–176, 2020.
- [10] D. Johannsmann, I. Reviakine, and R. P. Richter. Dissipation in films of adsorbed nanospheres studied by quartz crystal microbalance (QCM). *Analytical Chemistry*, 81(19):8167–8176, 2009.
- [11] J. J. J. Gillissen, J. A. Jackman, S. R. Tabaei, B. K. Yoon, and N.-J. Cho. Quartz crystal microbalance model for quantitatively probing the deformation of adsorbed particles at low surface coverage. *Analytical Chemistry*, 89(21):11711–11718, 2017.
- [12] L. Daikhin and M. Urbakh. Effect of surface film structure on the quartz crystal microbalance response in liquids. *Langmuir*, 12(26):6354–6360, 1996.
- [13] L. Daikhin, E. Gileadi, G. Katz, V. Tsionsky, M. Urbakh, and Z. Dmitriy. Influence of roughness on the admittance of the quartz crystal microbalance immersed in liquids. *Analytical Chemistry*, 74(3):554–561, 2002.
- [14] B. Liedberg, I. Lundström, and E. Stenberg. Principles of biosensing with an extended coupling matrix and surface plasmon resonance. *Sensors and Actuators: B. Chemical*, 11(1-3):63–72, 1993.
- [15] L. S. Jung, C. T. Campbell, T. M. Chinowsky, M. N. Mar, and S. S. Yee. Quantitative interpretation of the response of surface plasmon resonance sensors to adsorbed films. *Langmuir*, 14(19):5636–5648, 1998.
- [16] G. Ferrand-Drake Del Castillo, G. Emilsson, and A. Dahlin. Quantitative analysis of thickness and pH actuation of weak polyelectrolyte brushes. *Journal of Physical Chemistry C*, 122(48):27516–27527, 2018.
- [17] D. L.M. Rupert, G. V. Shelke, G. Emilsson, V. Claudio, S. Block, C. Lässer, A. Dahlin, J. O. Lötvall, M. Bally, V. P. Zhdanov, and F. Höök. Dual-wavelength surface plasmon resonance for determining the size and concentration of sub-populations of extracellular vesicles. *Analytical Chemistry*, 88(20):9980–9988, 2016.
- [18] M. J. Avena and L. K. Koopal. Desorption of humic acids from an iron oxide surface. *Environmental Science and Technology*, 32(17):2572–2577, 1998.
